# Supplementary material for: Towards Multi-Objective Statistically Fair Federated Learning
Source: arXiv:2201.09917 source file (2022-01-24)
Supplement: Supplementary file 1 [file 7-appendix.tex]

\section{Appendix}
\begin{table*}[h]
\centering
\begin{tabular}{cccccccccc} \hline
Data & Number Epochs & Learning Rate & Initial Step & Step Size  \\ \hline
Adult&150&0.1&2&1.5\\ \hline
Health&350&0.1&0.001&10\\ \hline
\end{tabular}
\caption{Parameters used in the experiments for FedVal with 10 clients.}
\end{table*}

\begin{table*}[h]
\centering
\begin{tabular}{ccccc} \hline
Method&Data & Number of Rounds & Learning Rate & q \\ \hline
q-Fed&Adult&1000&0.01&5\\ \hline
q-Fed&Health&3000&0.01&5 \\ \hline
AFL&Adult&1000&0.01&0 \\ \hline
AFL&Health&3000&0.01&0 \\ \hline
\end{tabular}
\caption{Parameters used in the experiments for q-FedSGD, q-FedAvg, and AFL.}
\end{table*}

\begin{table*}[h]
\centering
\begin{tabular}{ccc} \hline
Data & Number of Epochs & Learning Rate \\ \hline
Adult&150&0.1 \\ \hline
Health&350&0.1 \\ \hline
\end{tabular}
\caption{Parameters used in the FedAvg experiments.}
\end{table*}

\begin{table*}[h]
\centering
\begin{tabular}{cccccc} \hline
Data & Number Epochs & Learning Rate & Initial Step & Step Size \\ \hline
Adult&150&0.1&2&1.5 \\ \hline
Health&150&0.1&2&1.5 \\ \hline
\end{tabular}
\caption{Parameters used in the experiments for FedVal with 100 clients.}
\end{table*}

\begin{figure*}[h]
\includegraphics[width=0.5\textwidth,trim=1cm 3cm 8cm 3cm,clip=true]{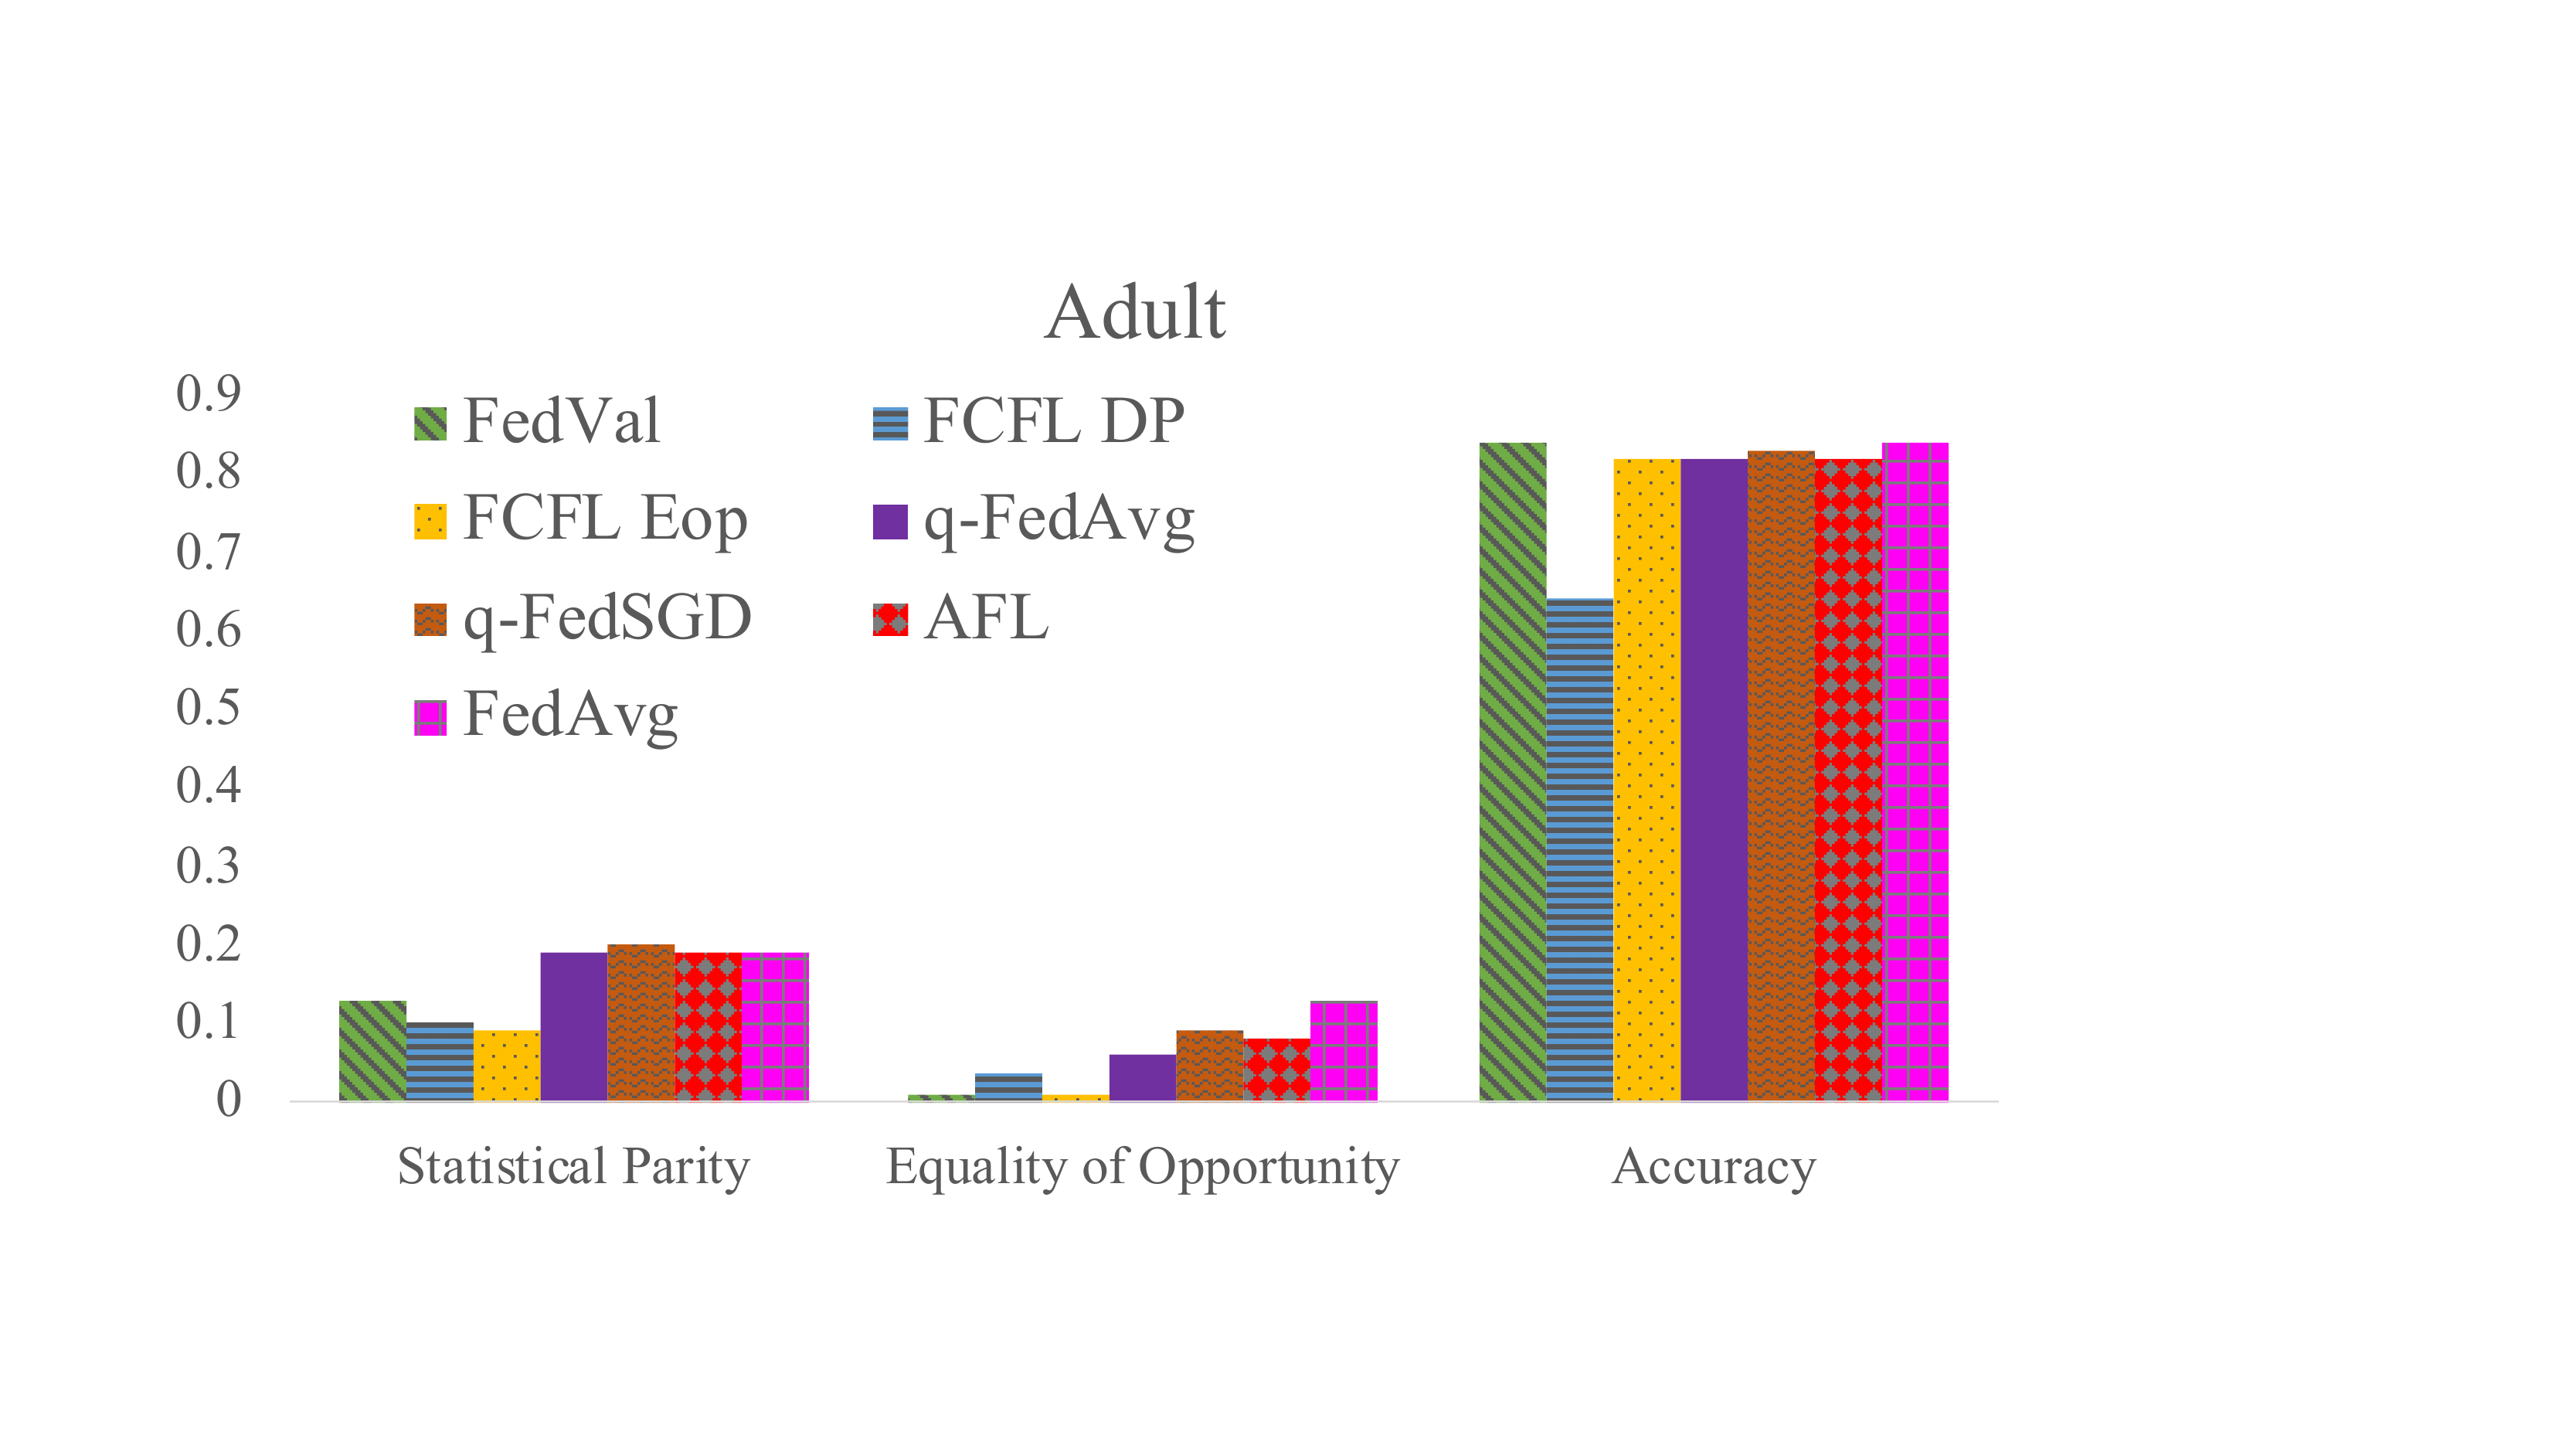}
\includegraphics[width=0.5\textwidth,trim=1cm 3cm 8cm 3cm,clip=true]{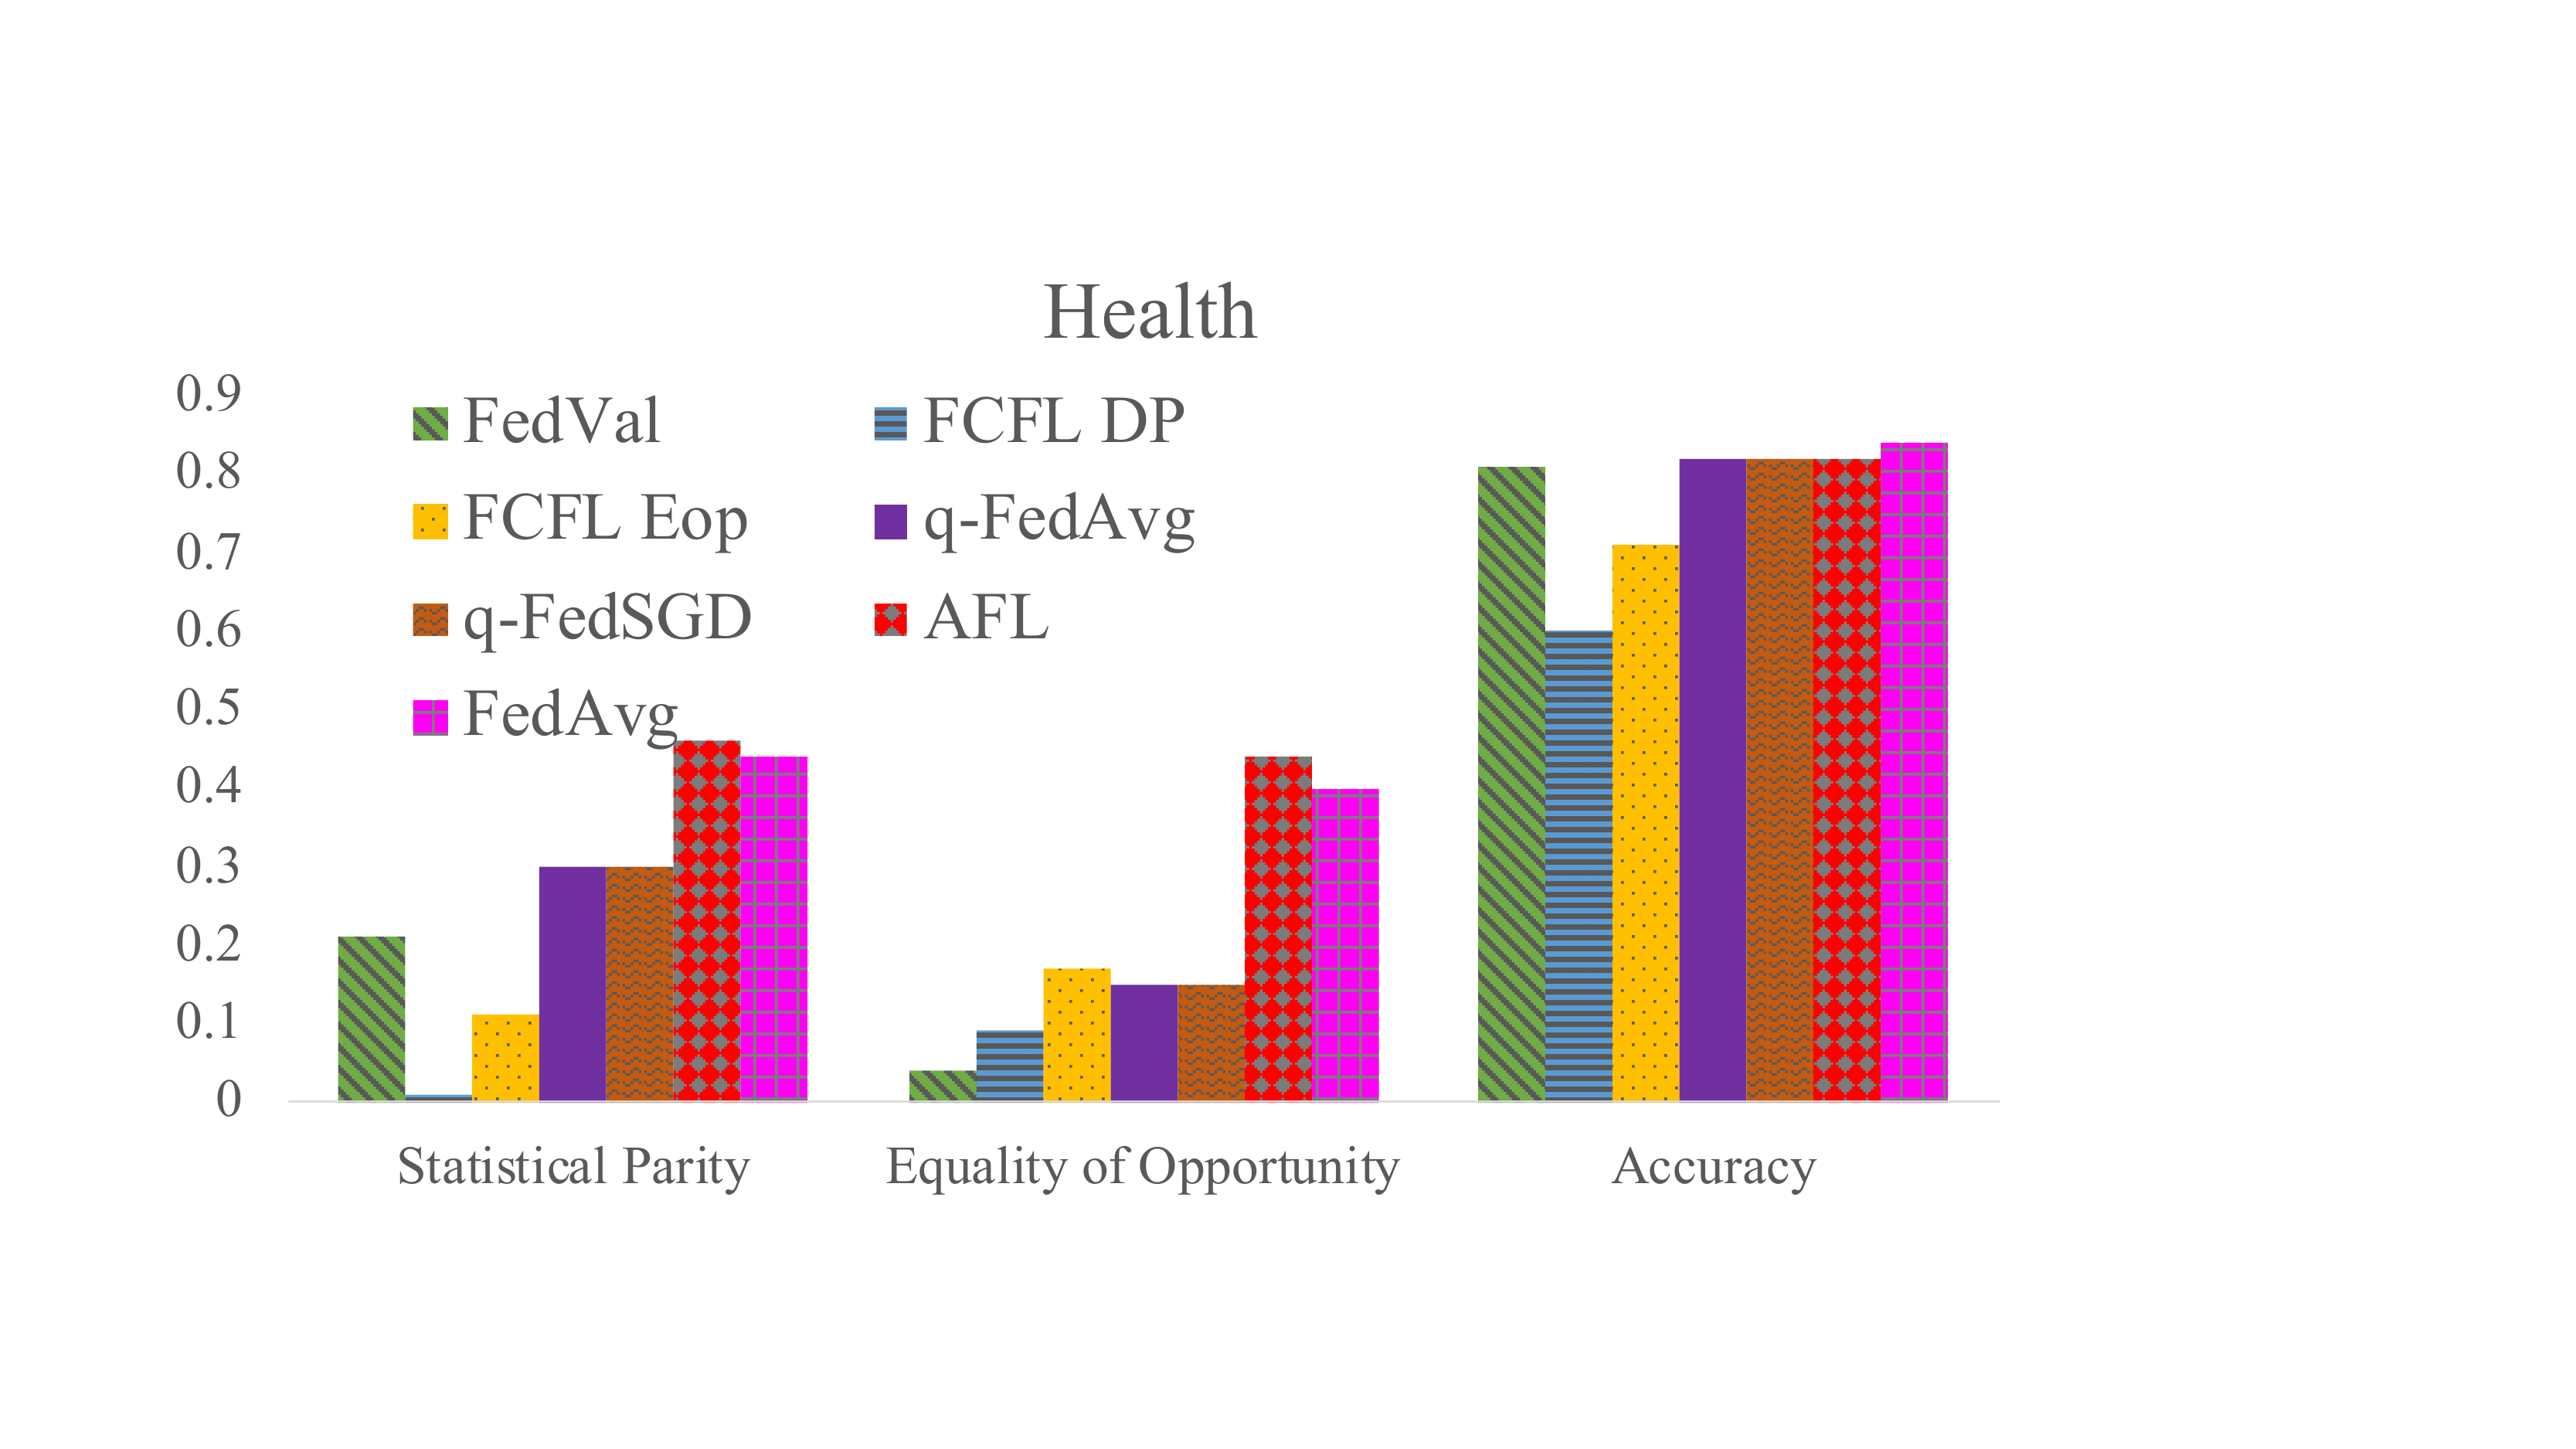}
\caption{FedVal compared to baselines in data regime one.}
\label{app-fig1}
\end{figure*}

\begin{figure*}[h]
\includegraphics[width=0.5\textwidth,trim=1cm 3cm 8cm 3cm,clip=true]{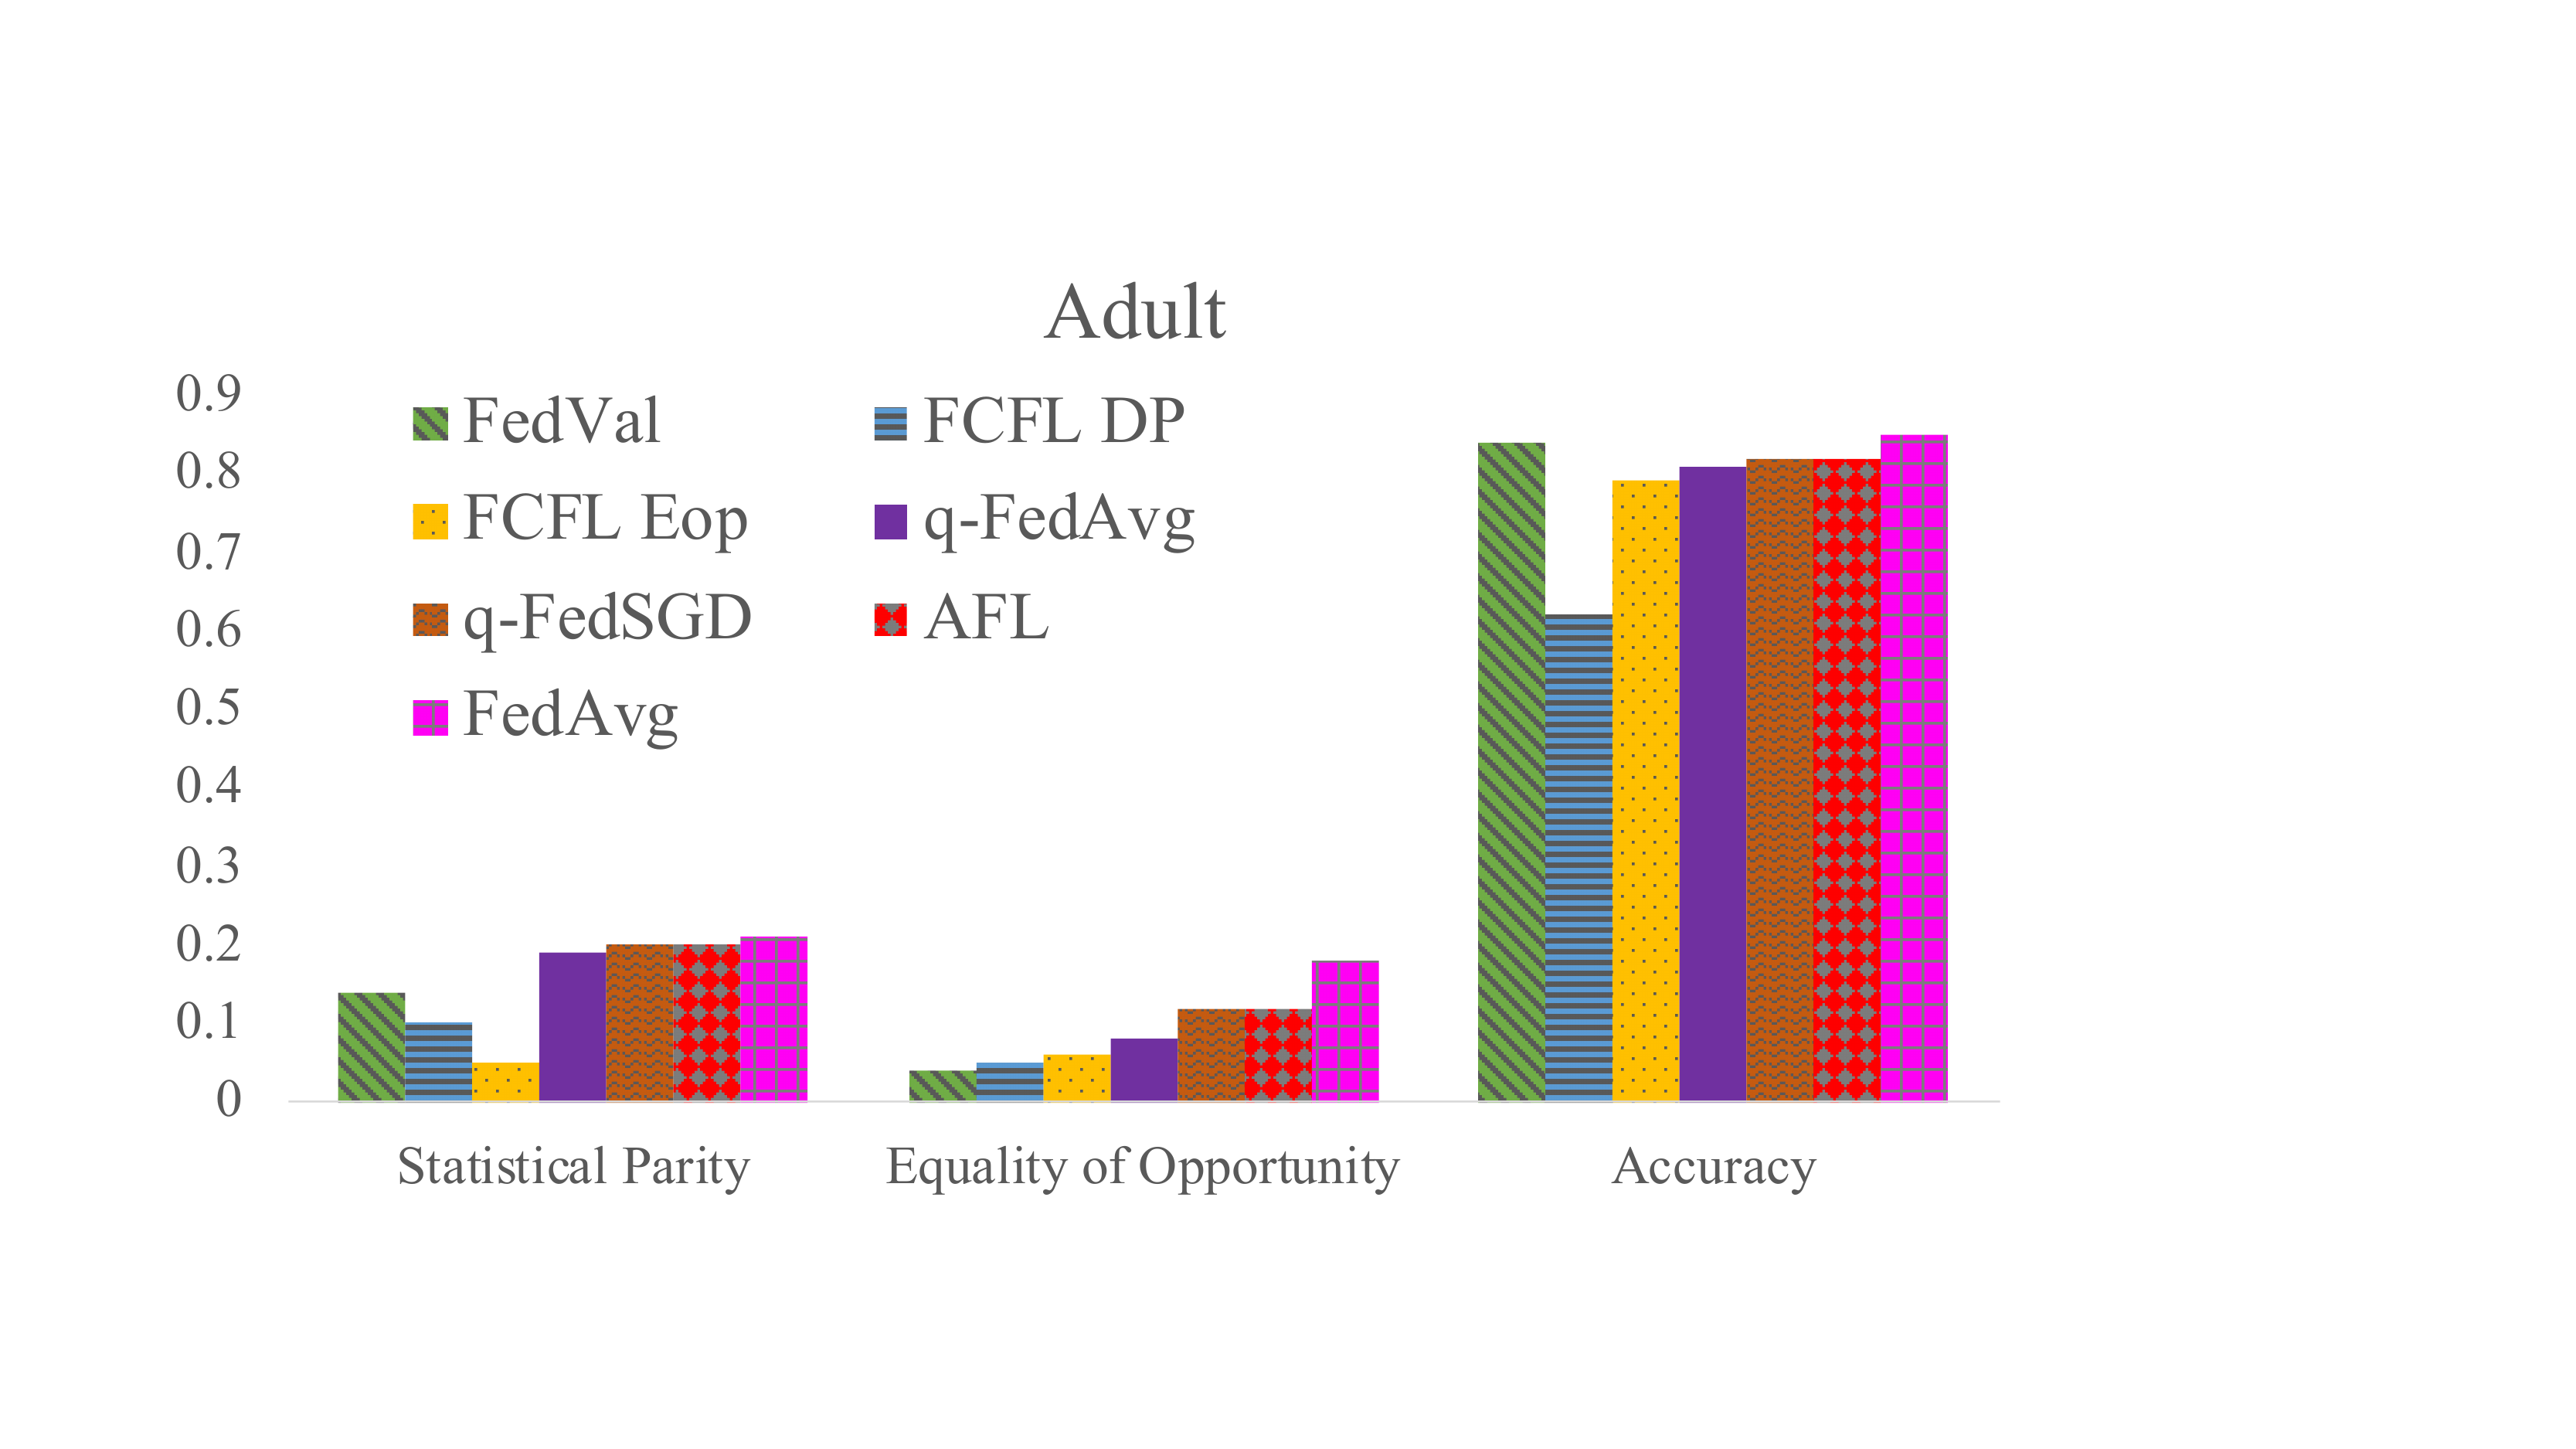}
\includegraphics[width=0.5\textwidth,trim=1cm 3cm 8cm 3cm,clip=true]{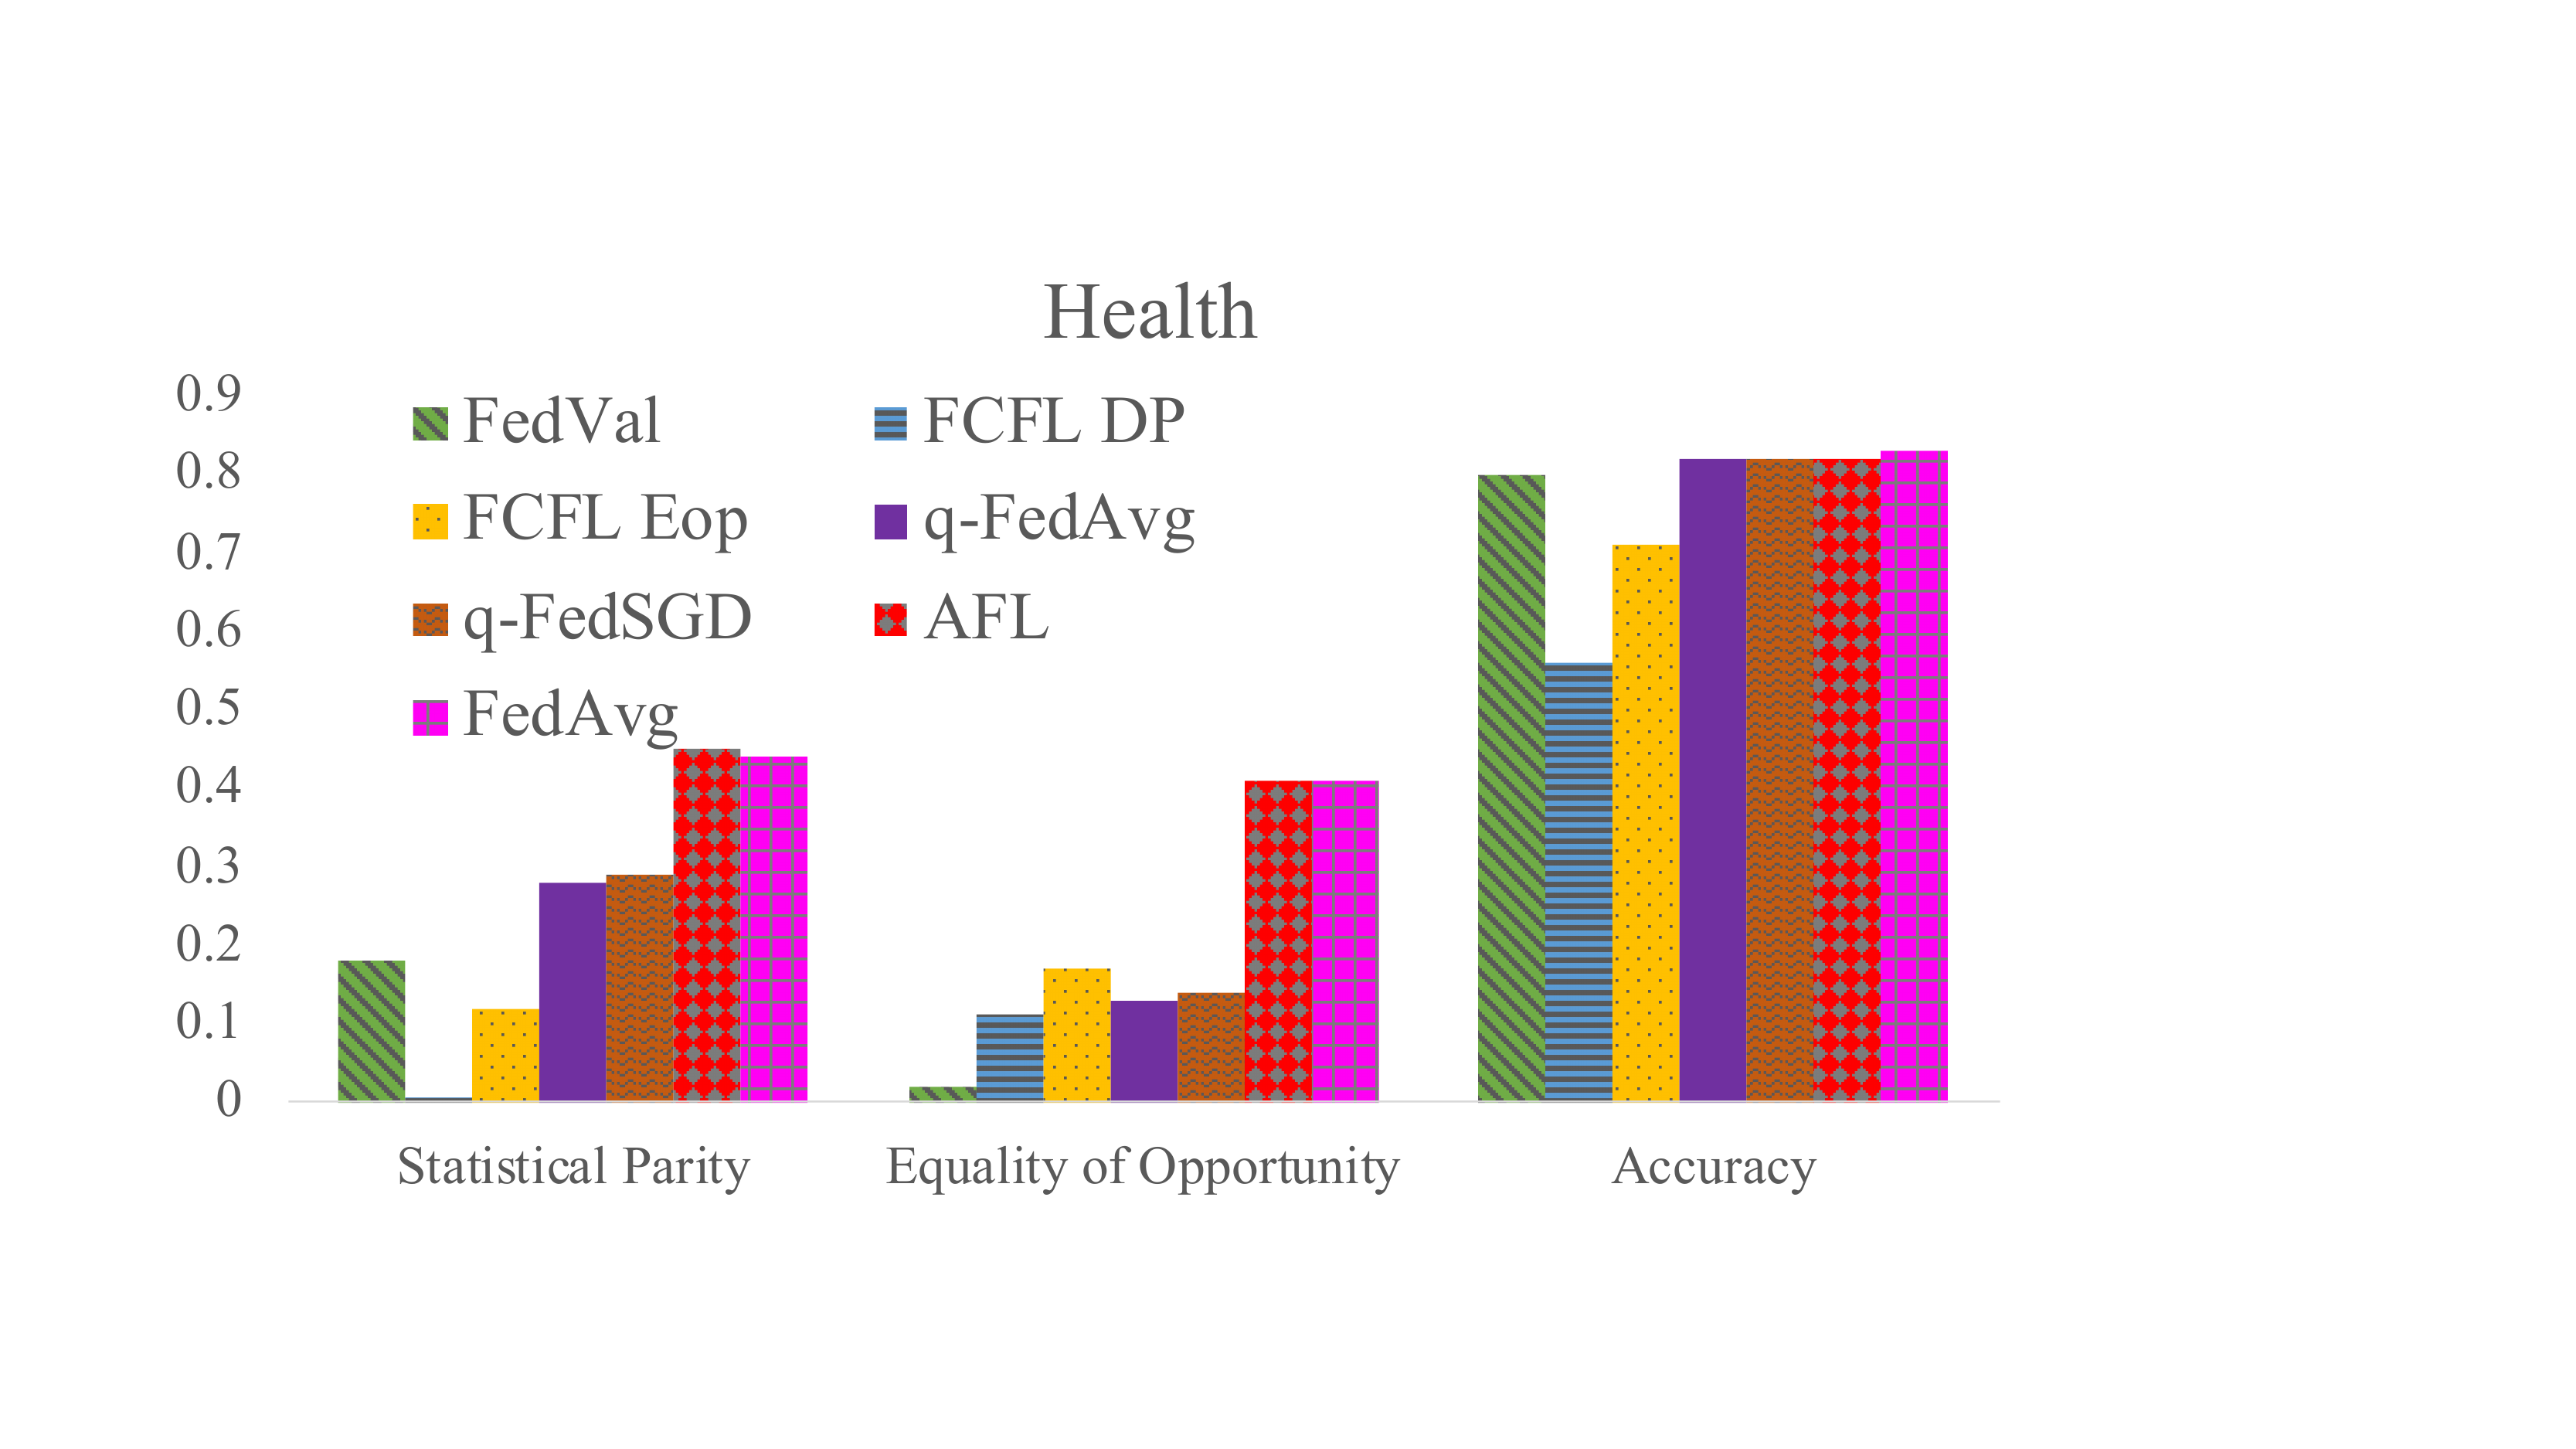}
\caption{FedVal compared to baselines in data regime two.}
\label{app-fig2}
\end{figure*}

\begin{figure*}[h]
\includegraphics[width=0.5\textwidth,trim=1cm 3cm 8cm 3cm,clip=true]{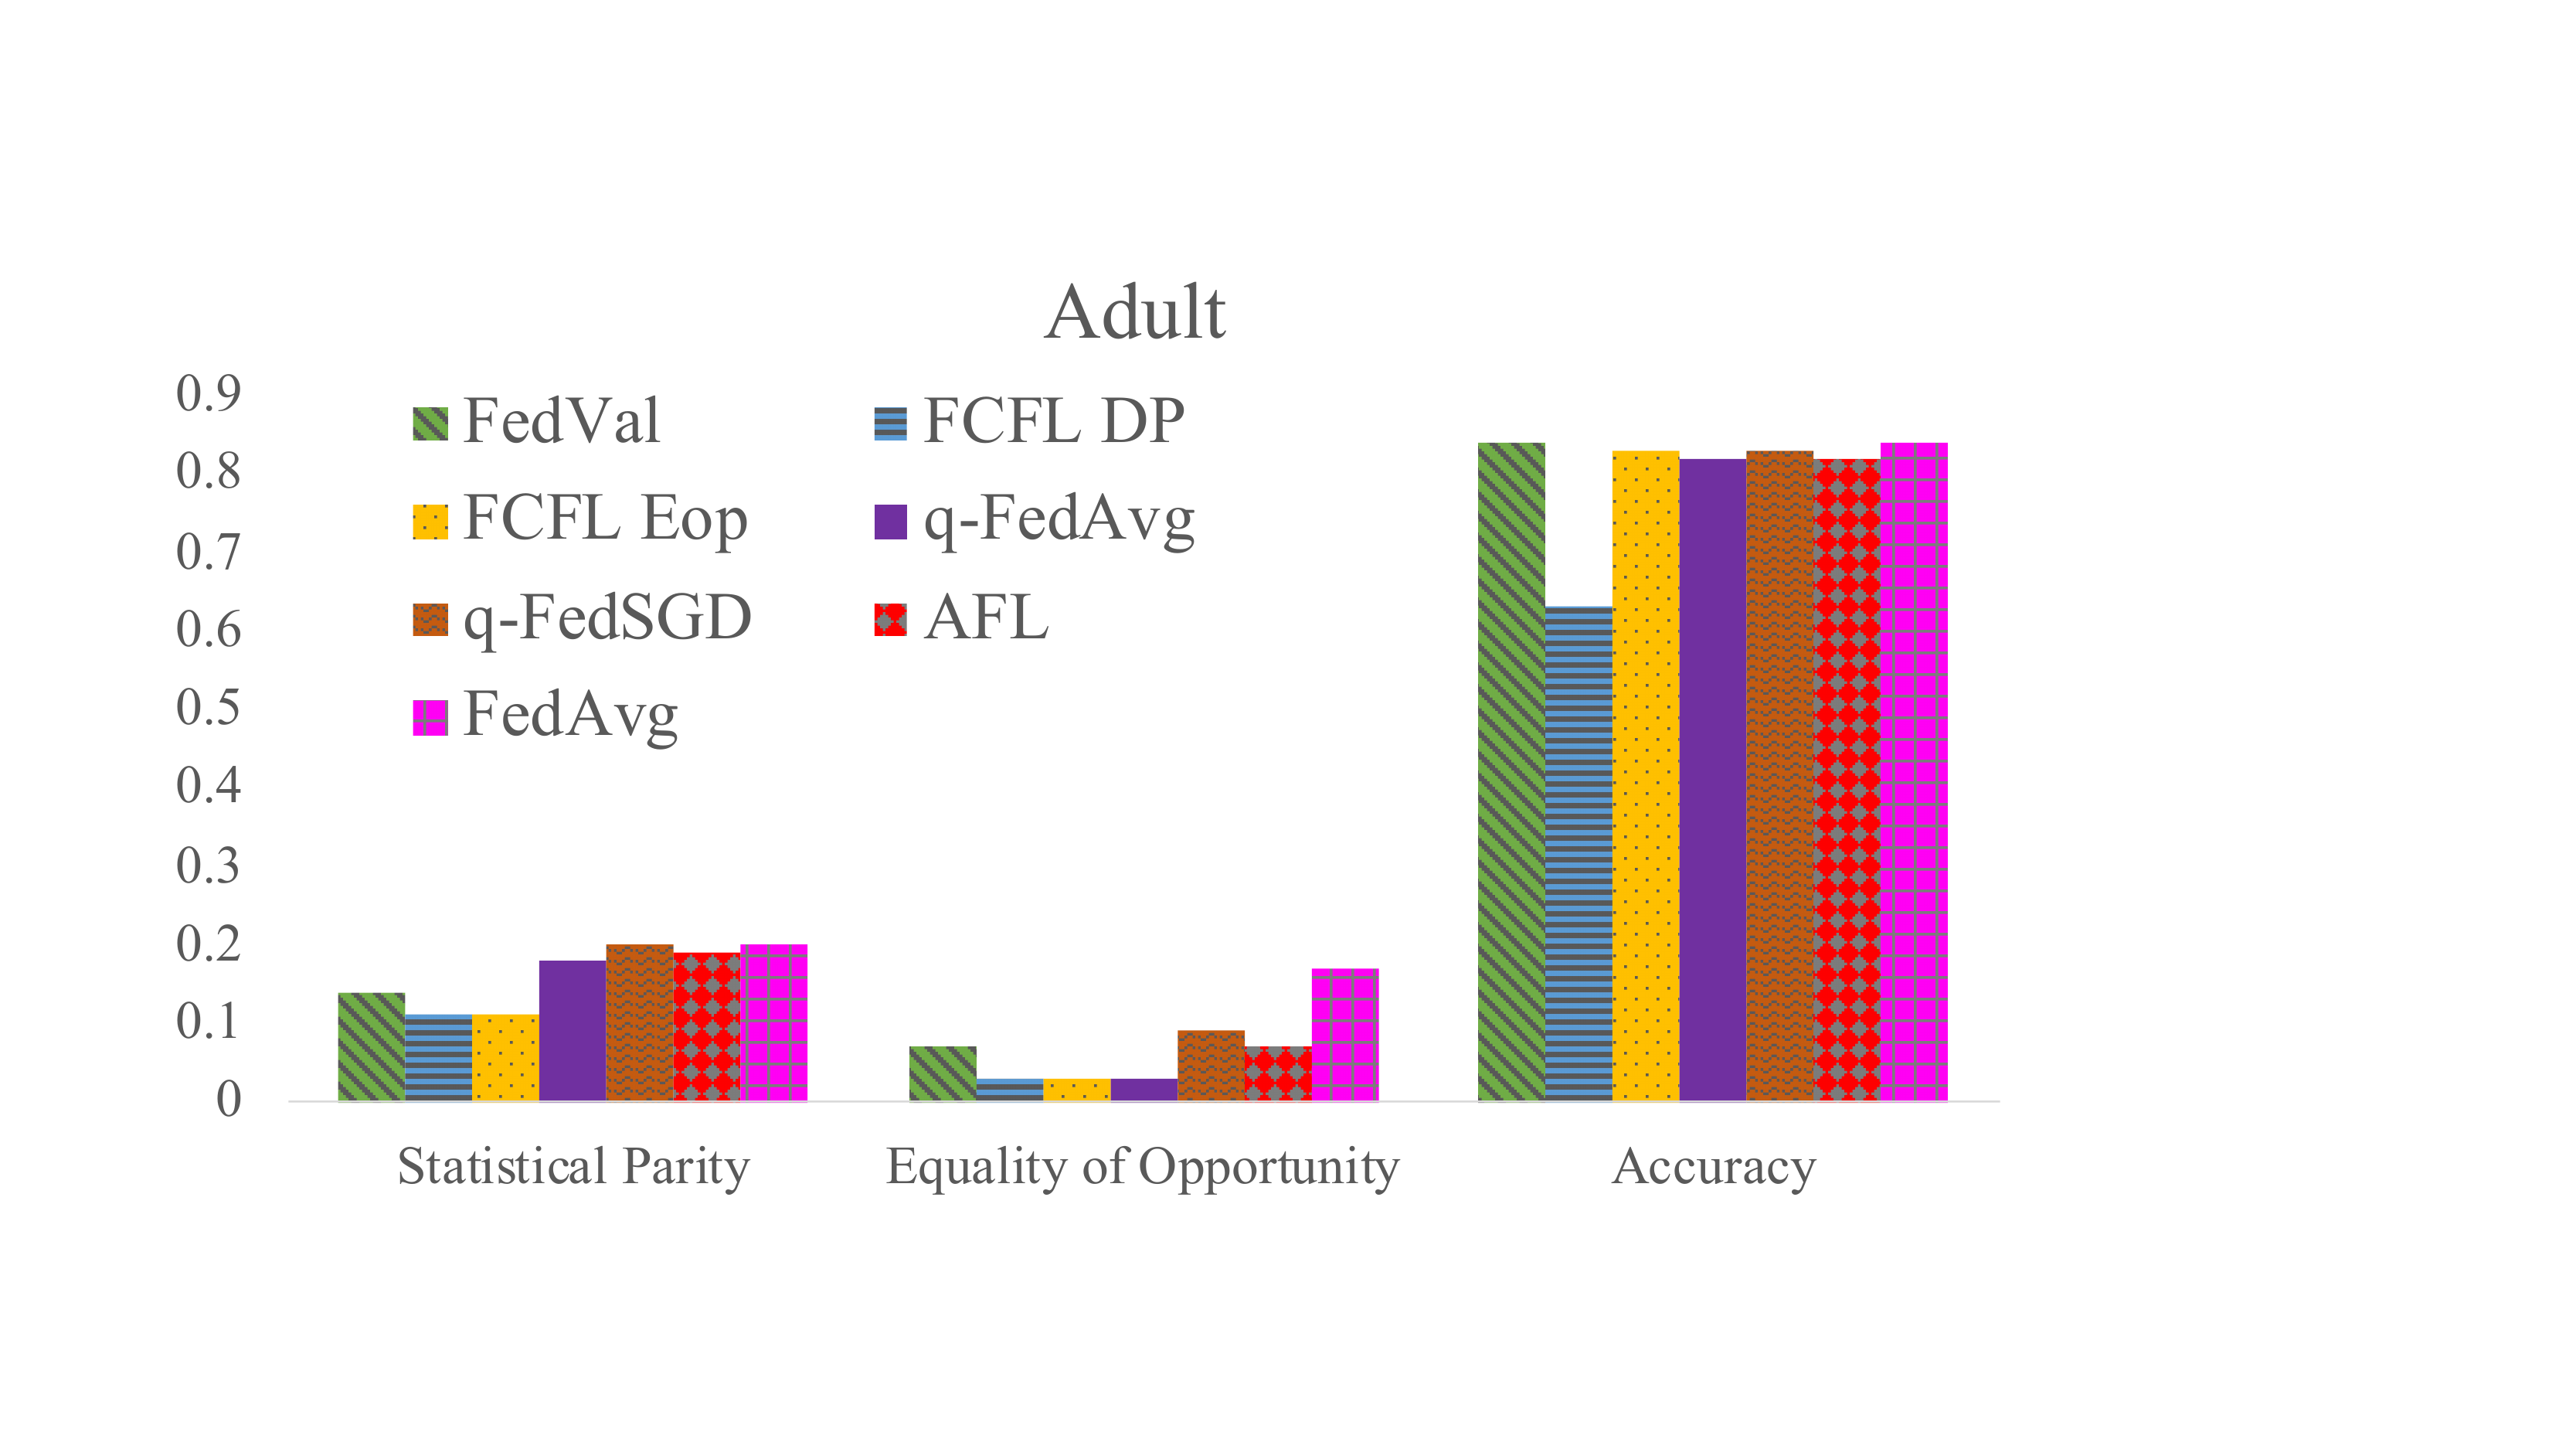}
\includegraphics[width=0.5\textwidth,trim=1cm 3cm 8cm 3cm,clip=true]{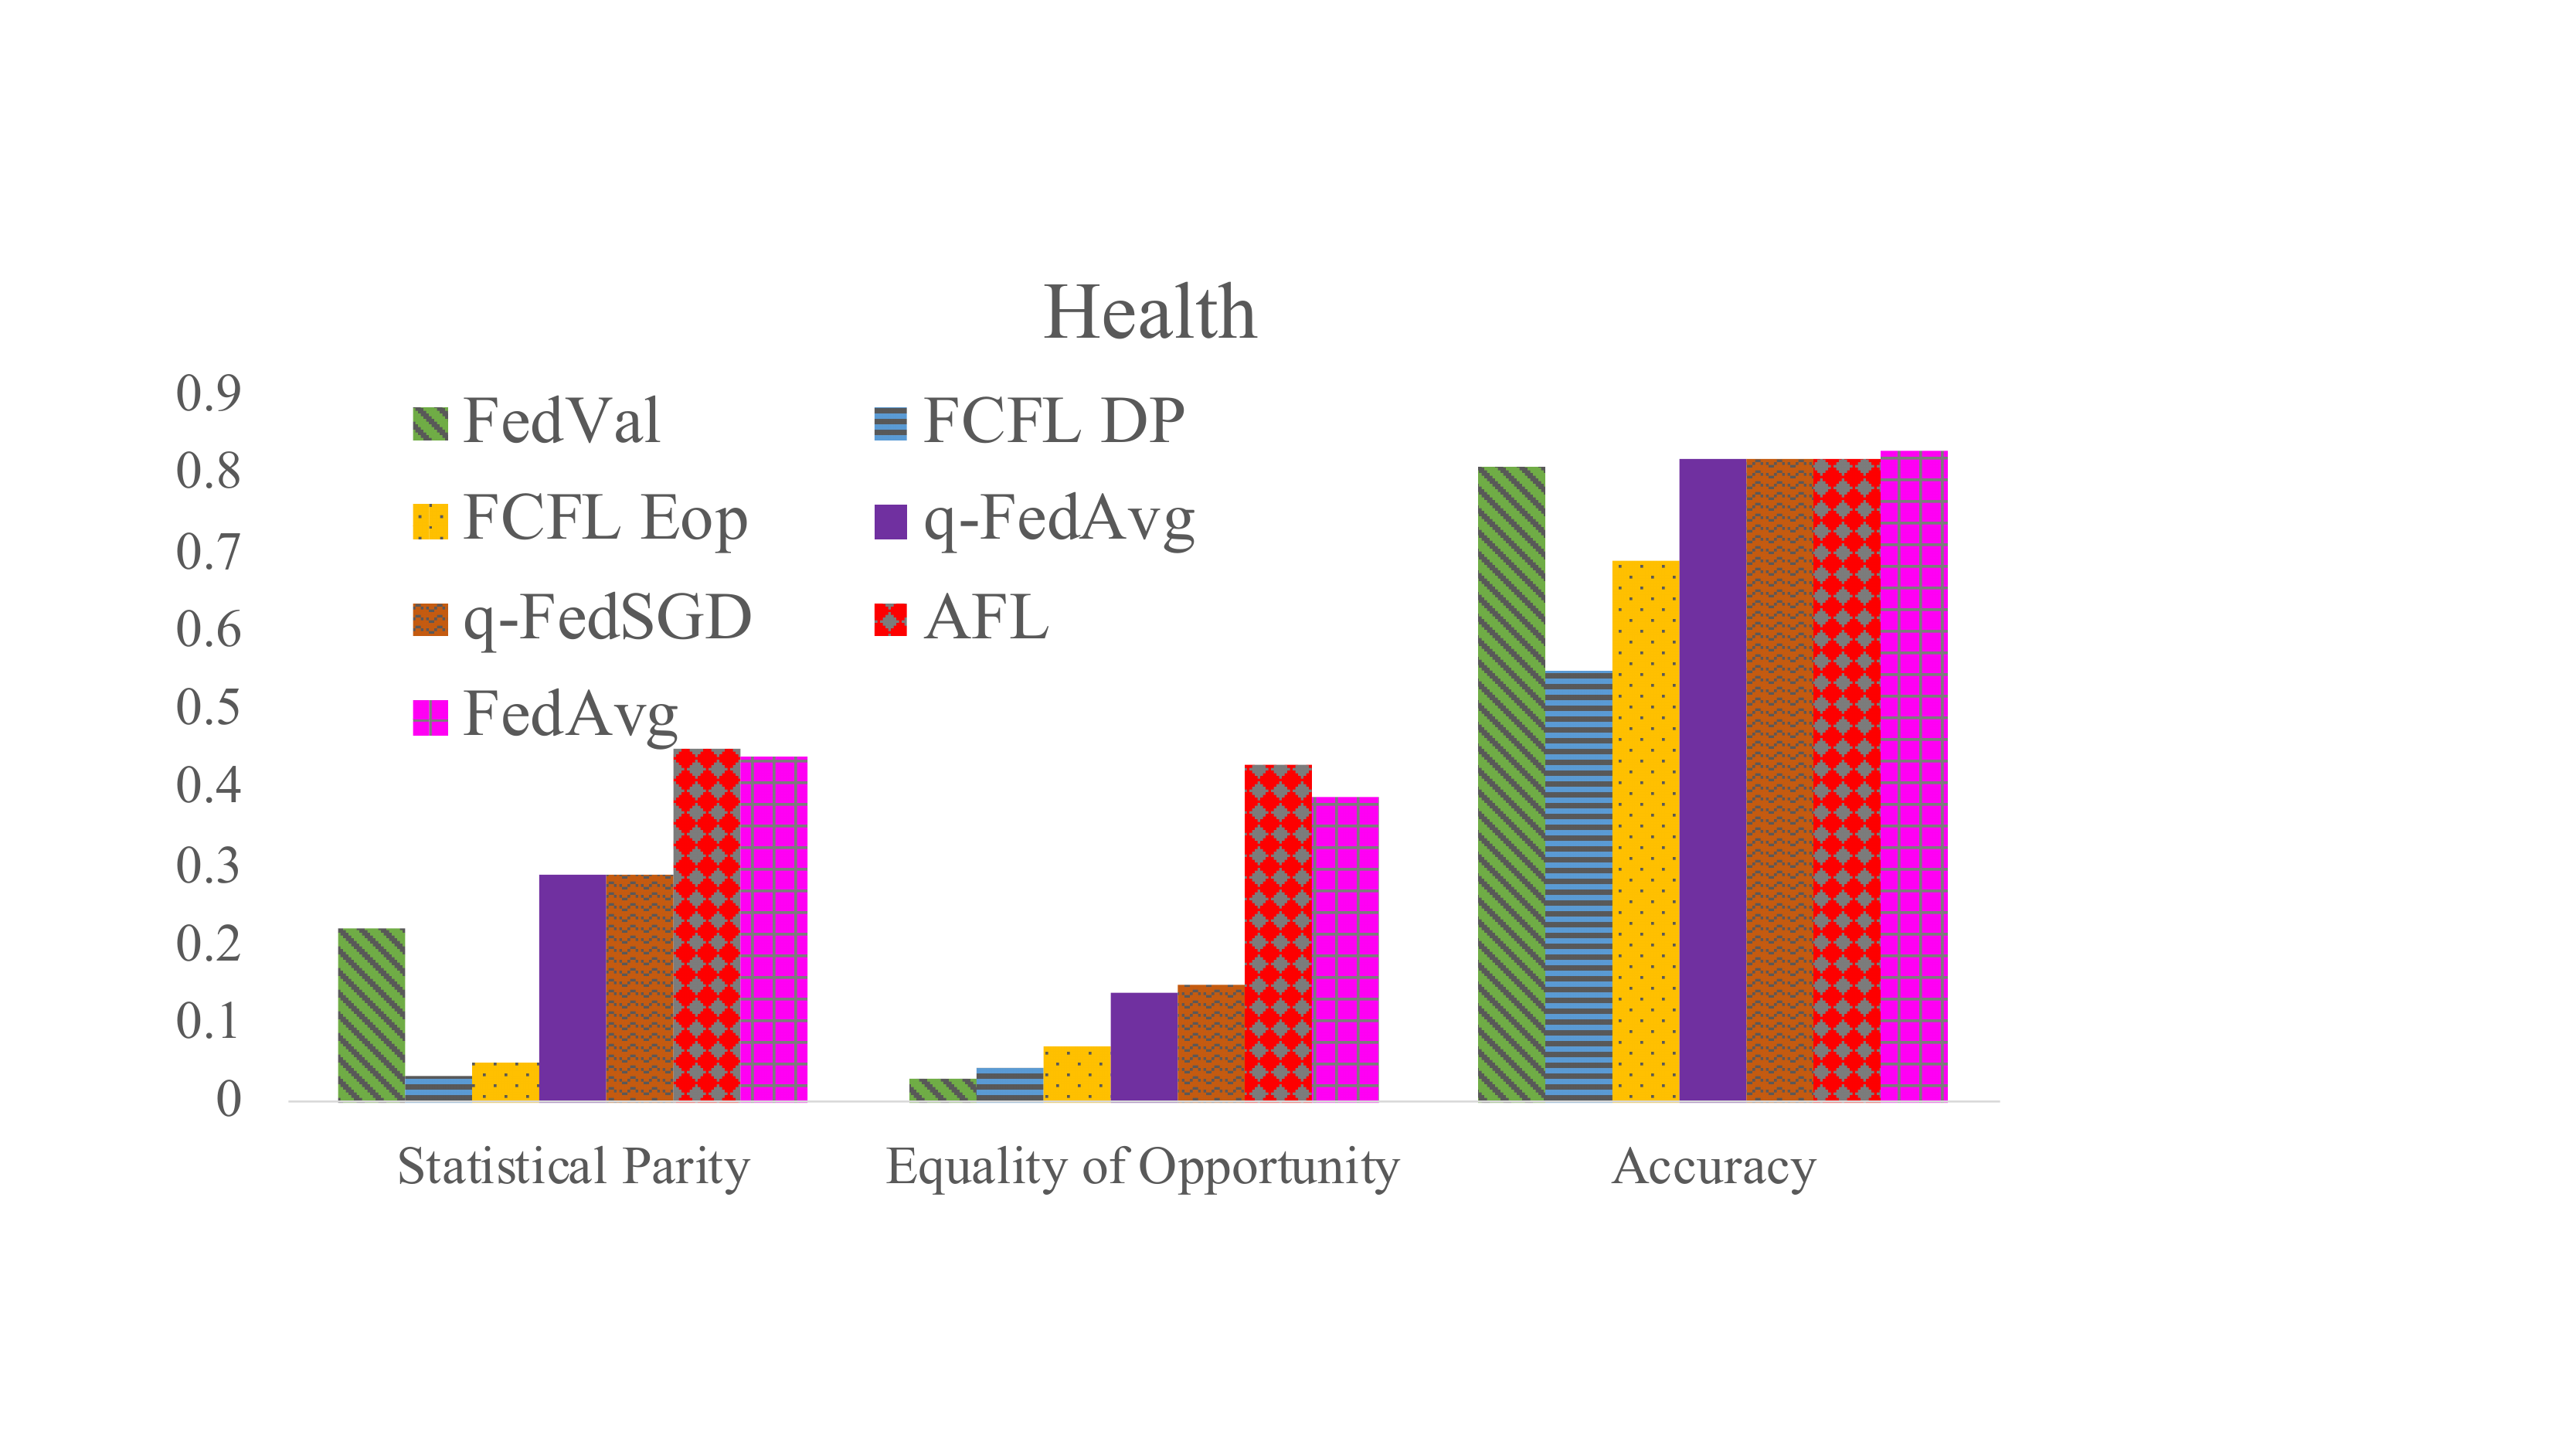}
\caption{FedVal compared to baselines in data regime three.}
\label{app-fig3}
\end{figure*}

\begin{figure*}[h]
\includegraphics[width=0.5\textwidth,trim=1cm 3cm 10cm 3cm,clip=true]{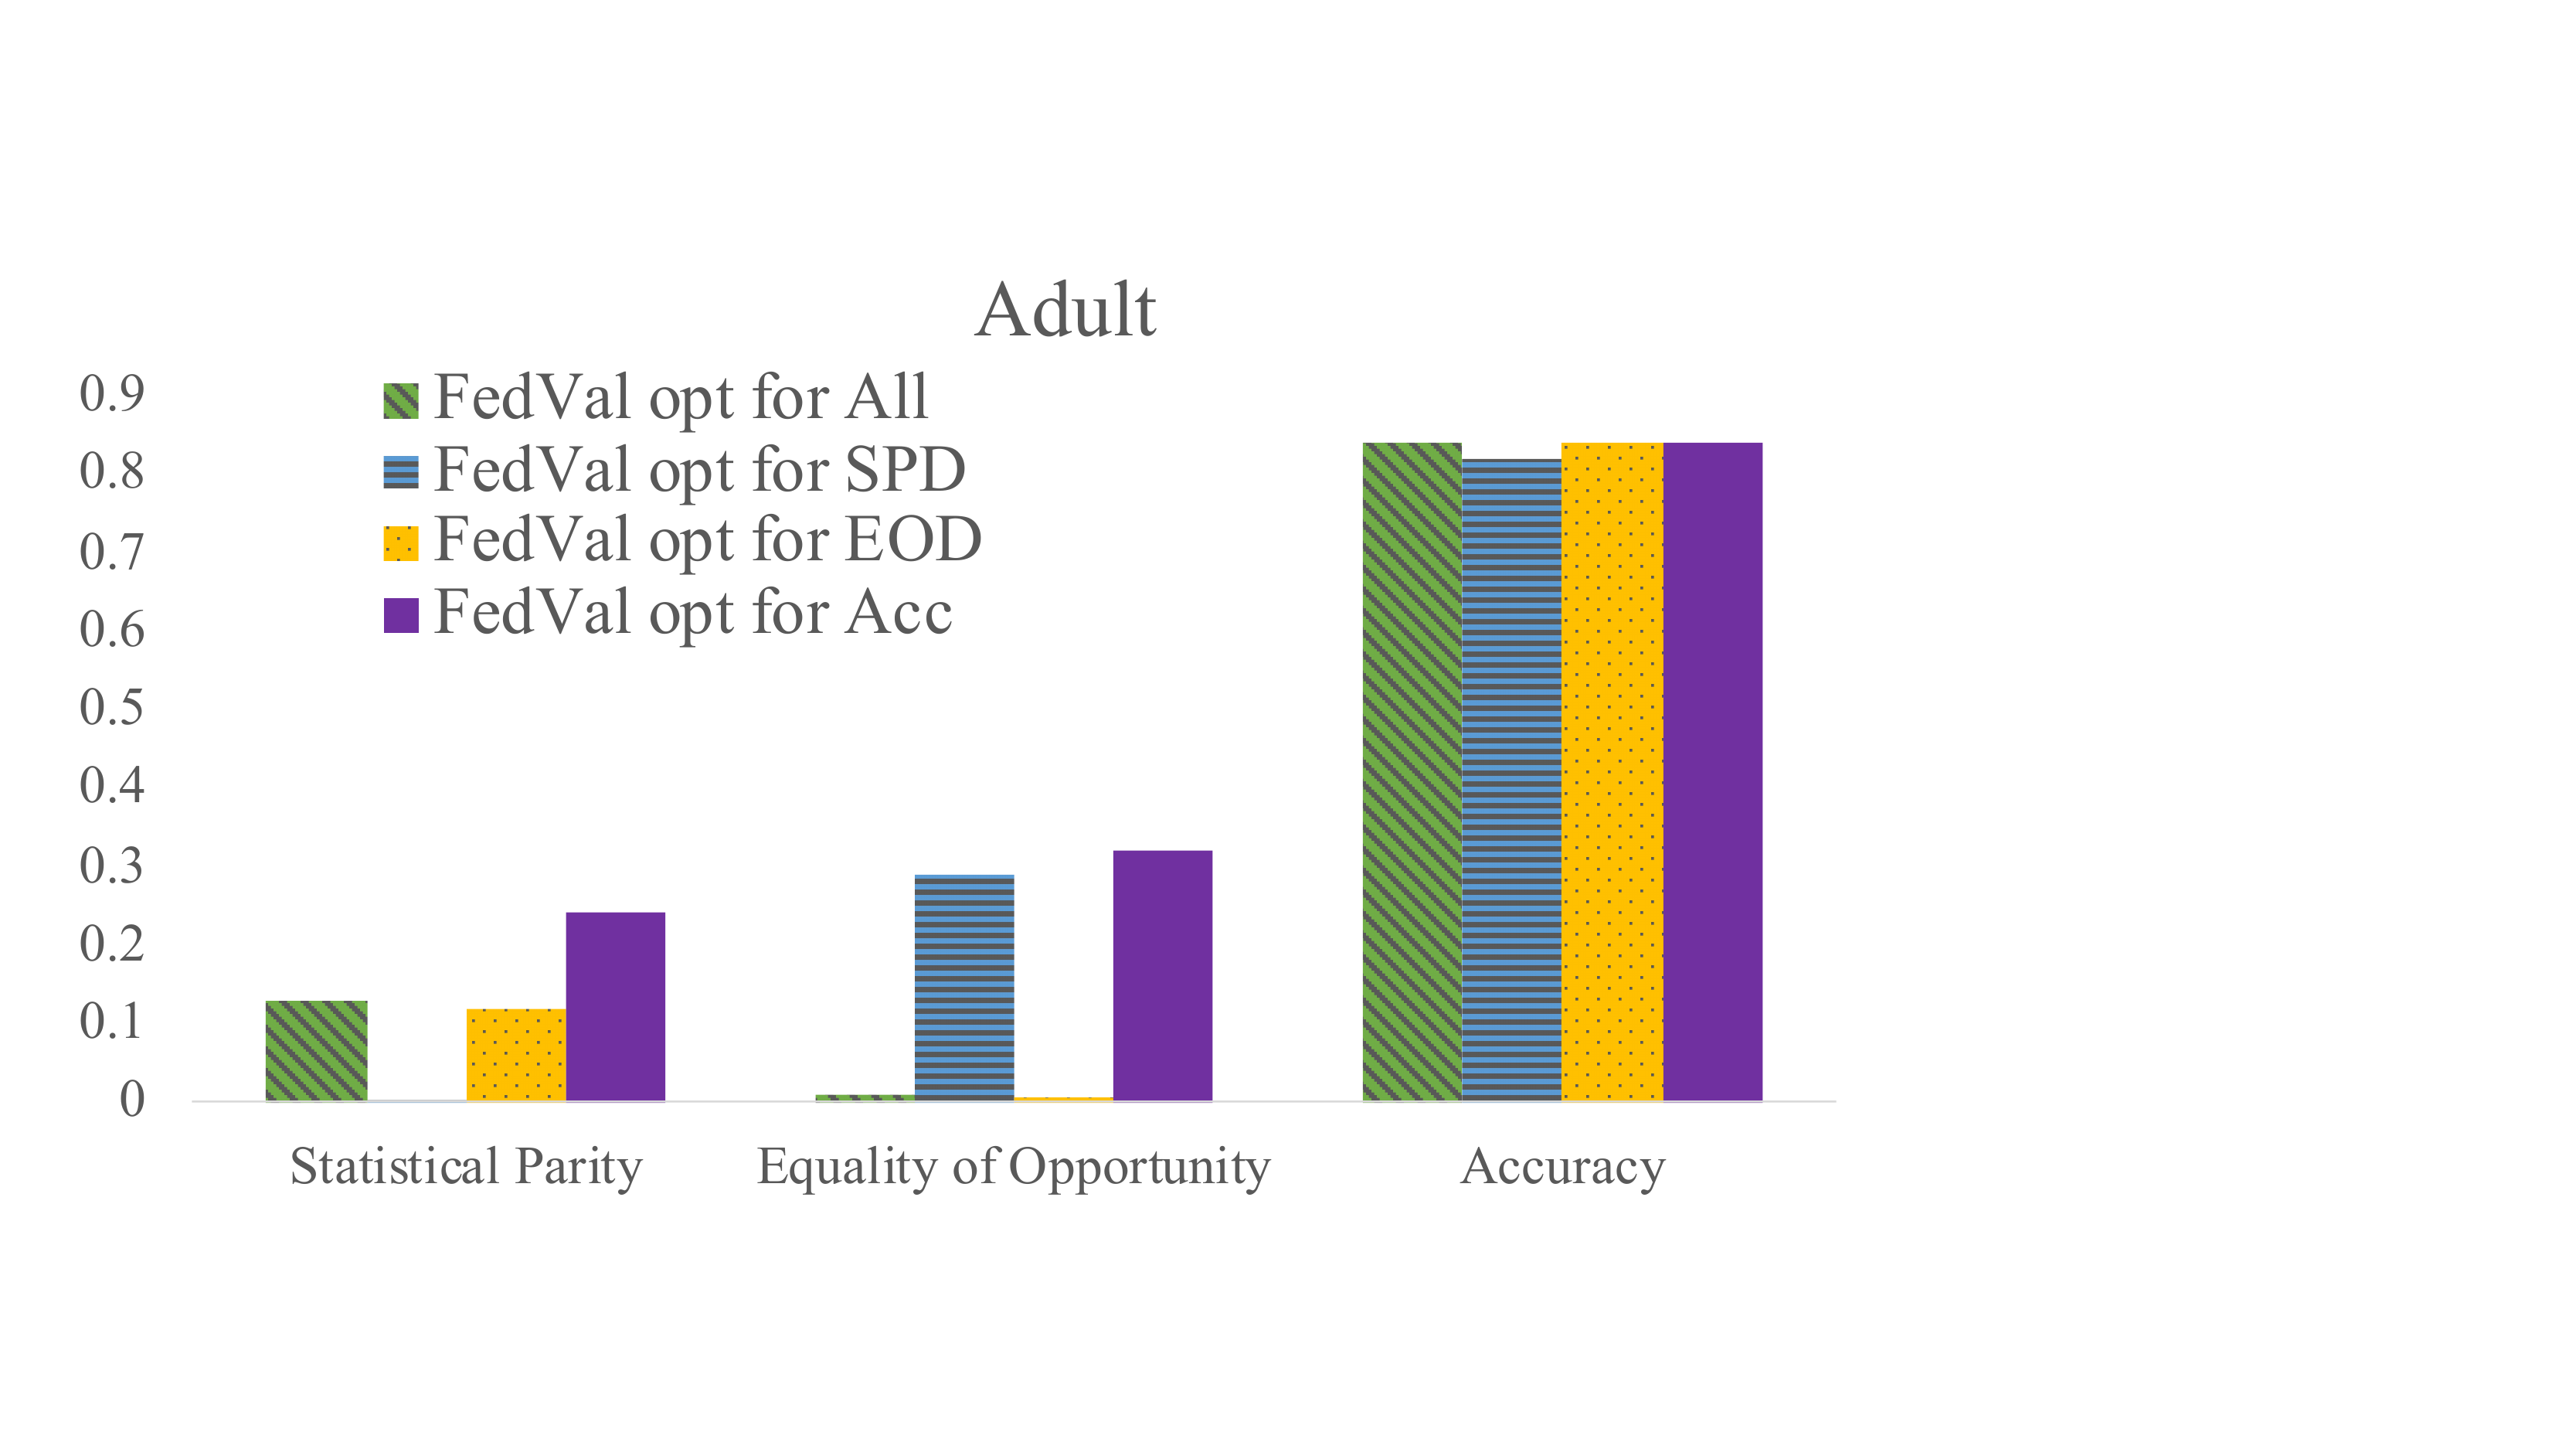}
\includegraphics[width=0.5\textwidth,trim=1cm 3cm 10cm 3cm,clip=true]{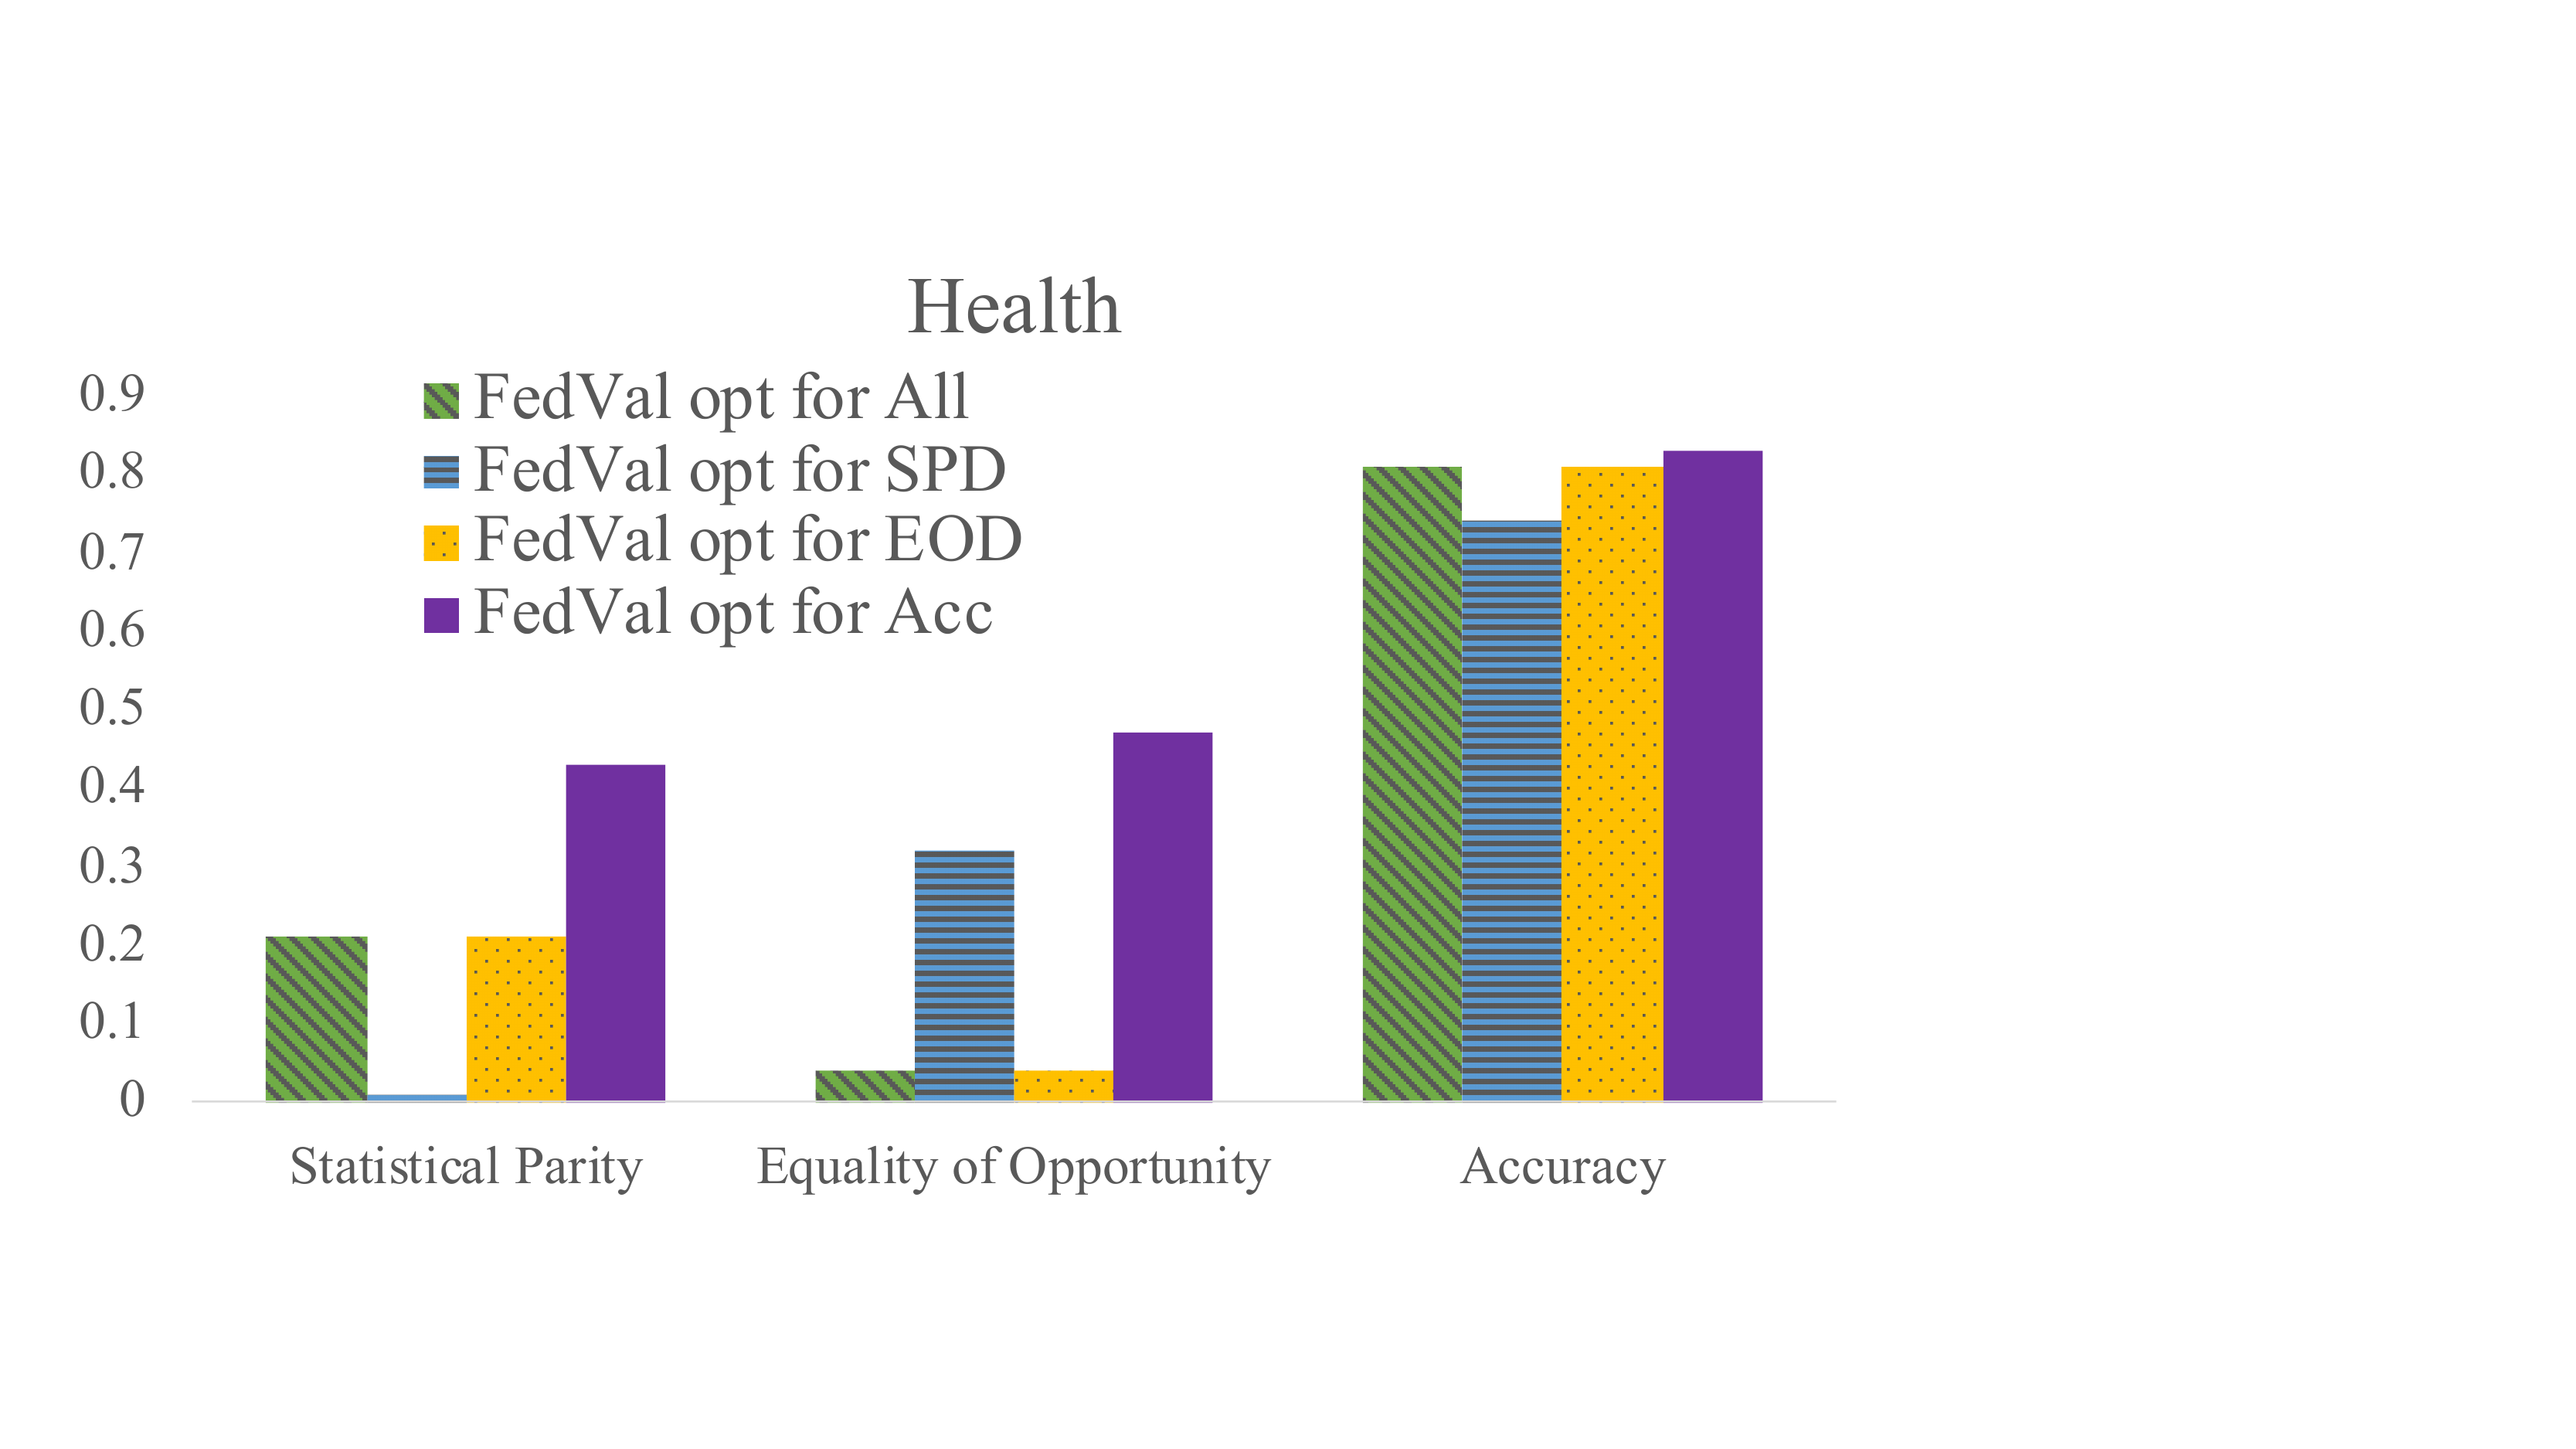}
\caption{FedVal optimized for different objectives in data regime one.}
\label{app-fig4}
\end{figure*}

\begin{figure*}[h]
\includegraphics[width=0.5\textwidth,trim=1cm 3cm 10cm 3cm,clip=true]{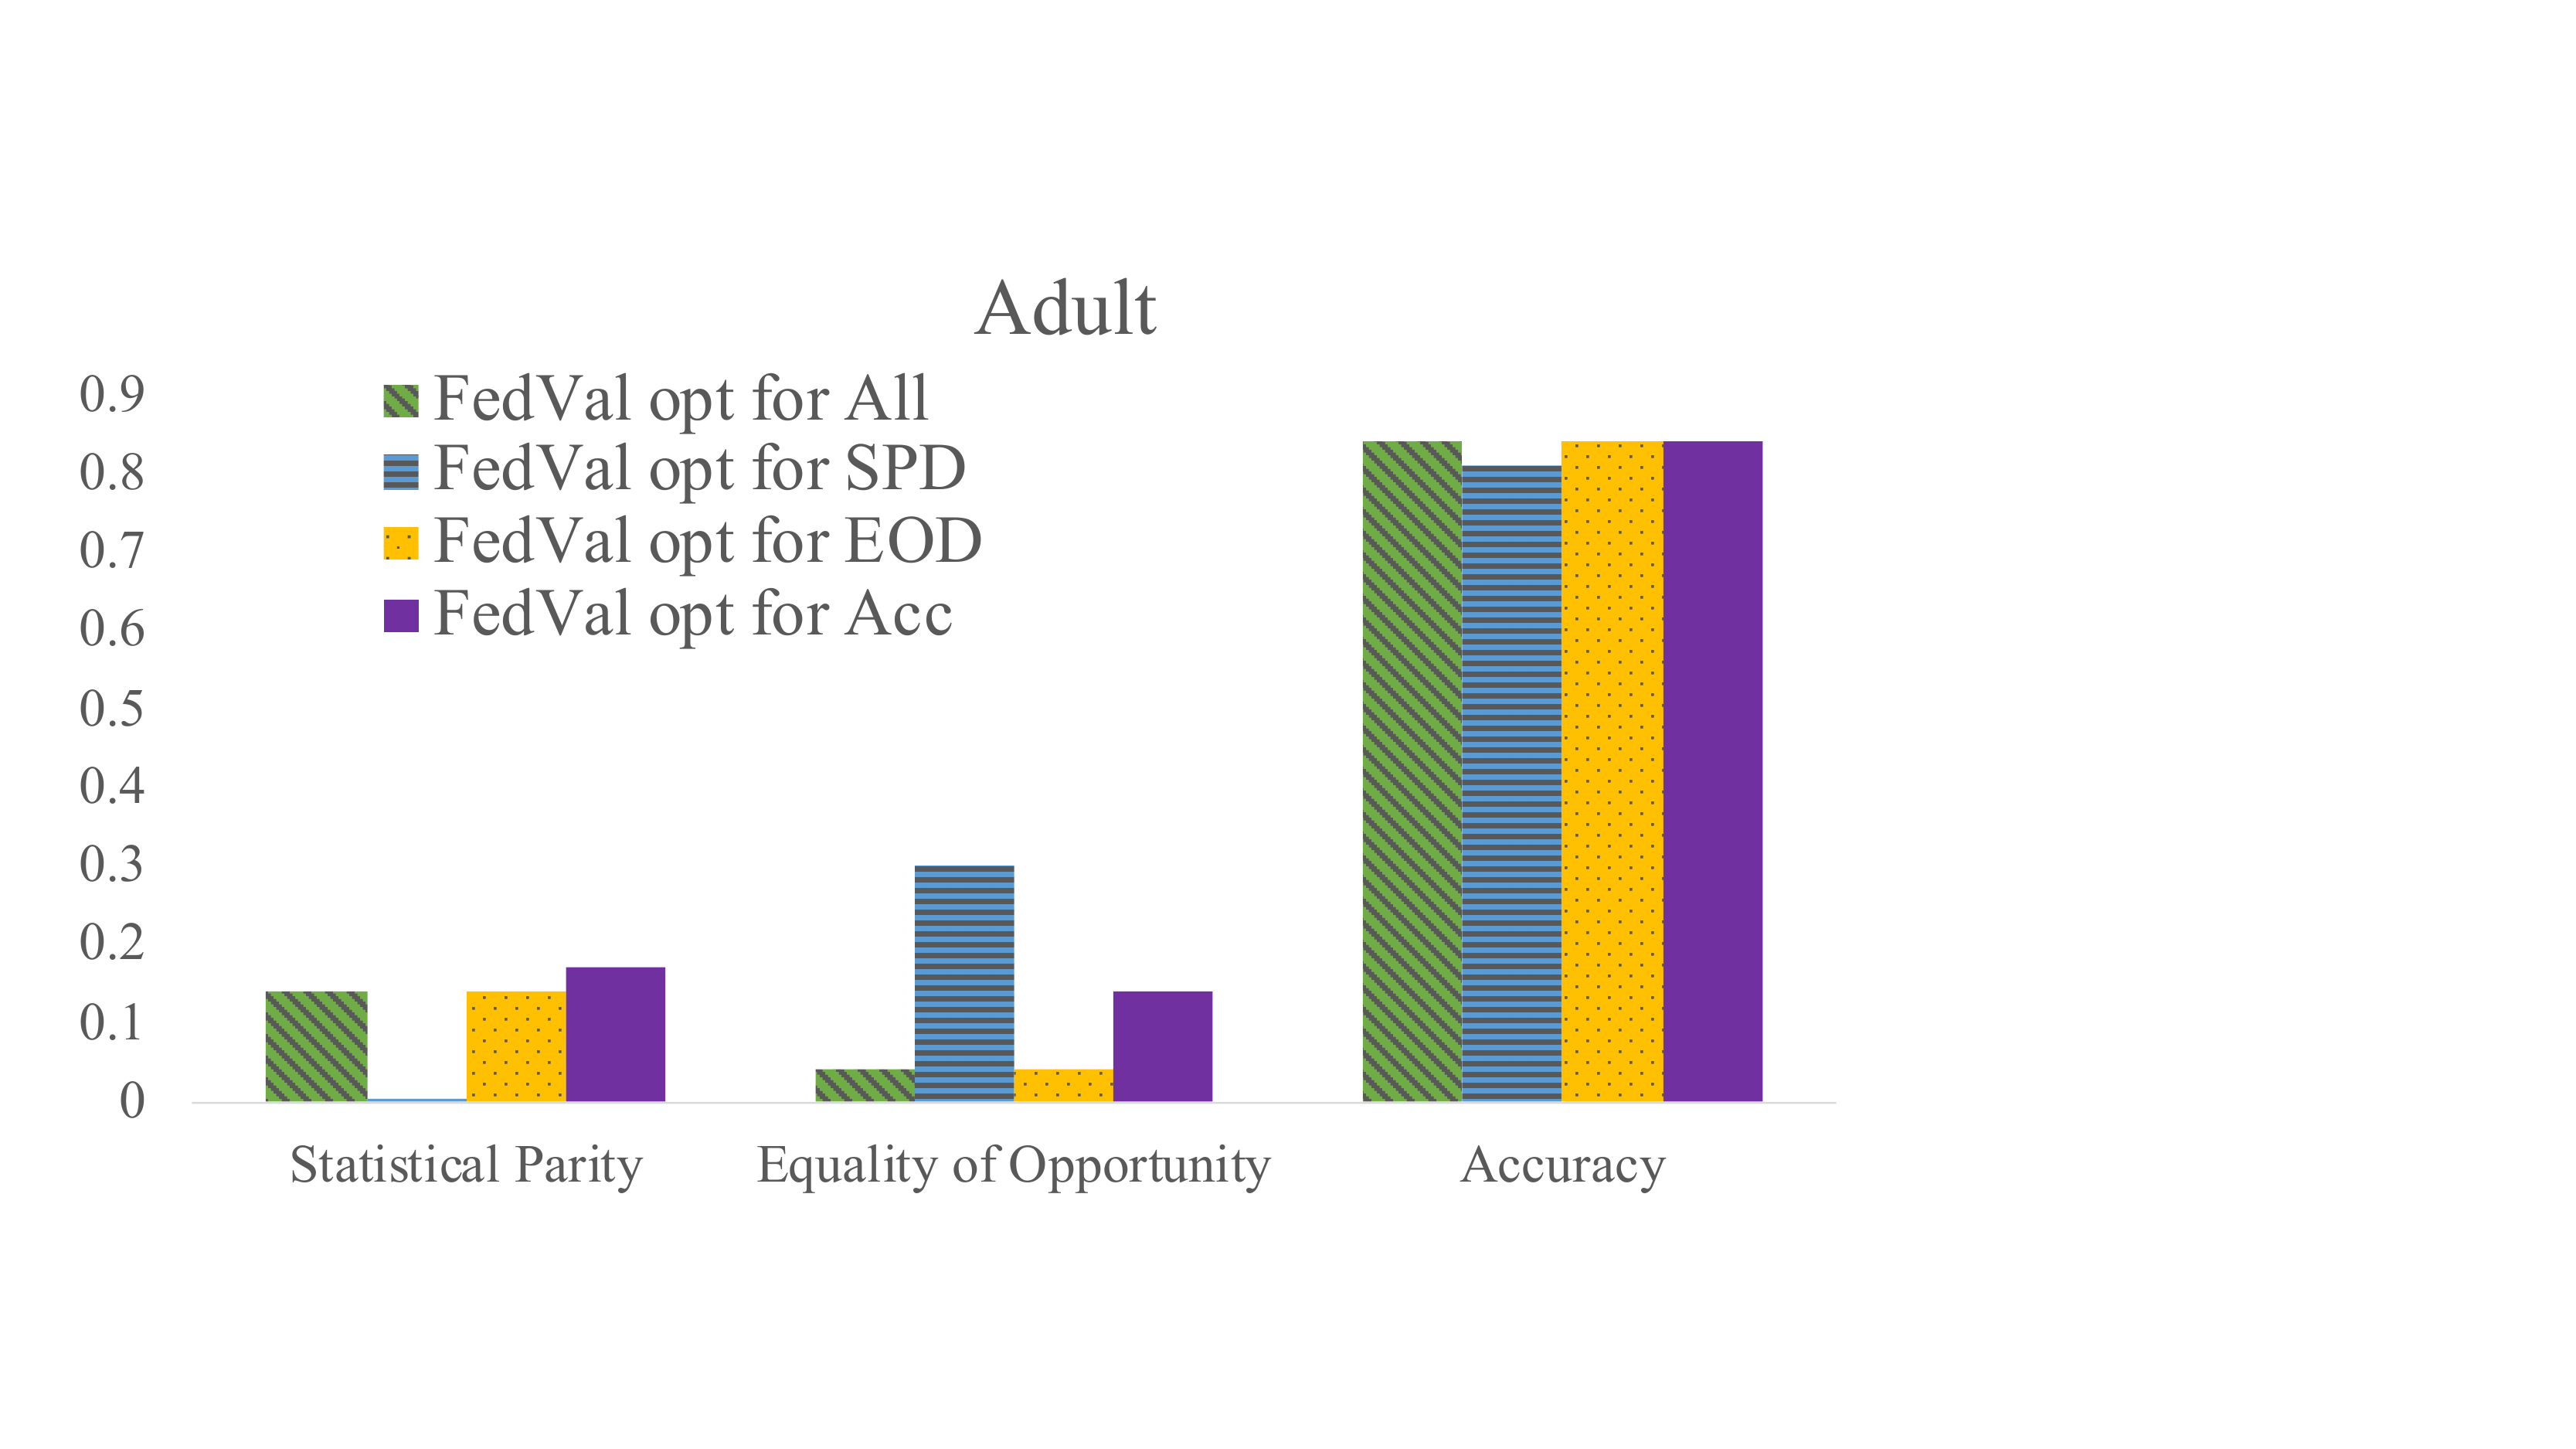}
\includegraphics[width=0.5\textwidth,trim=1cm 3cm 10cm 3cm,clip=true]{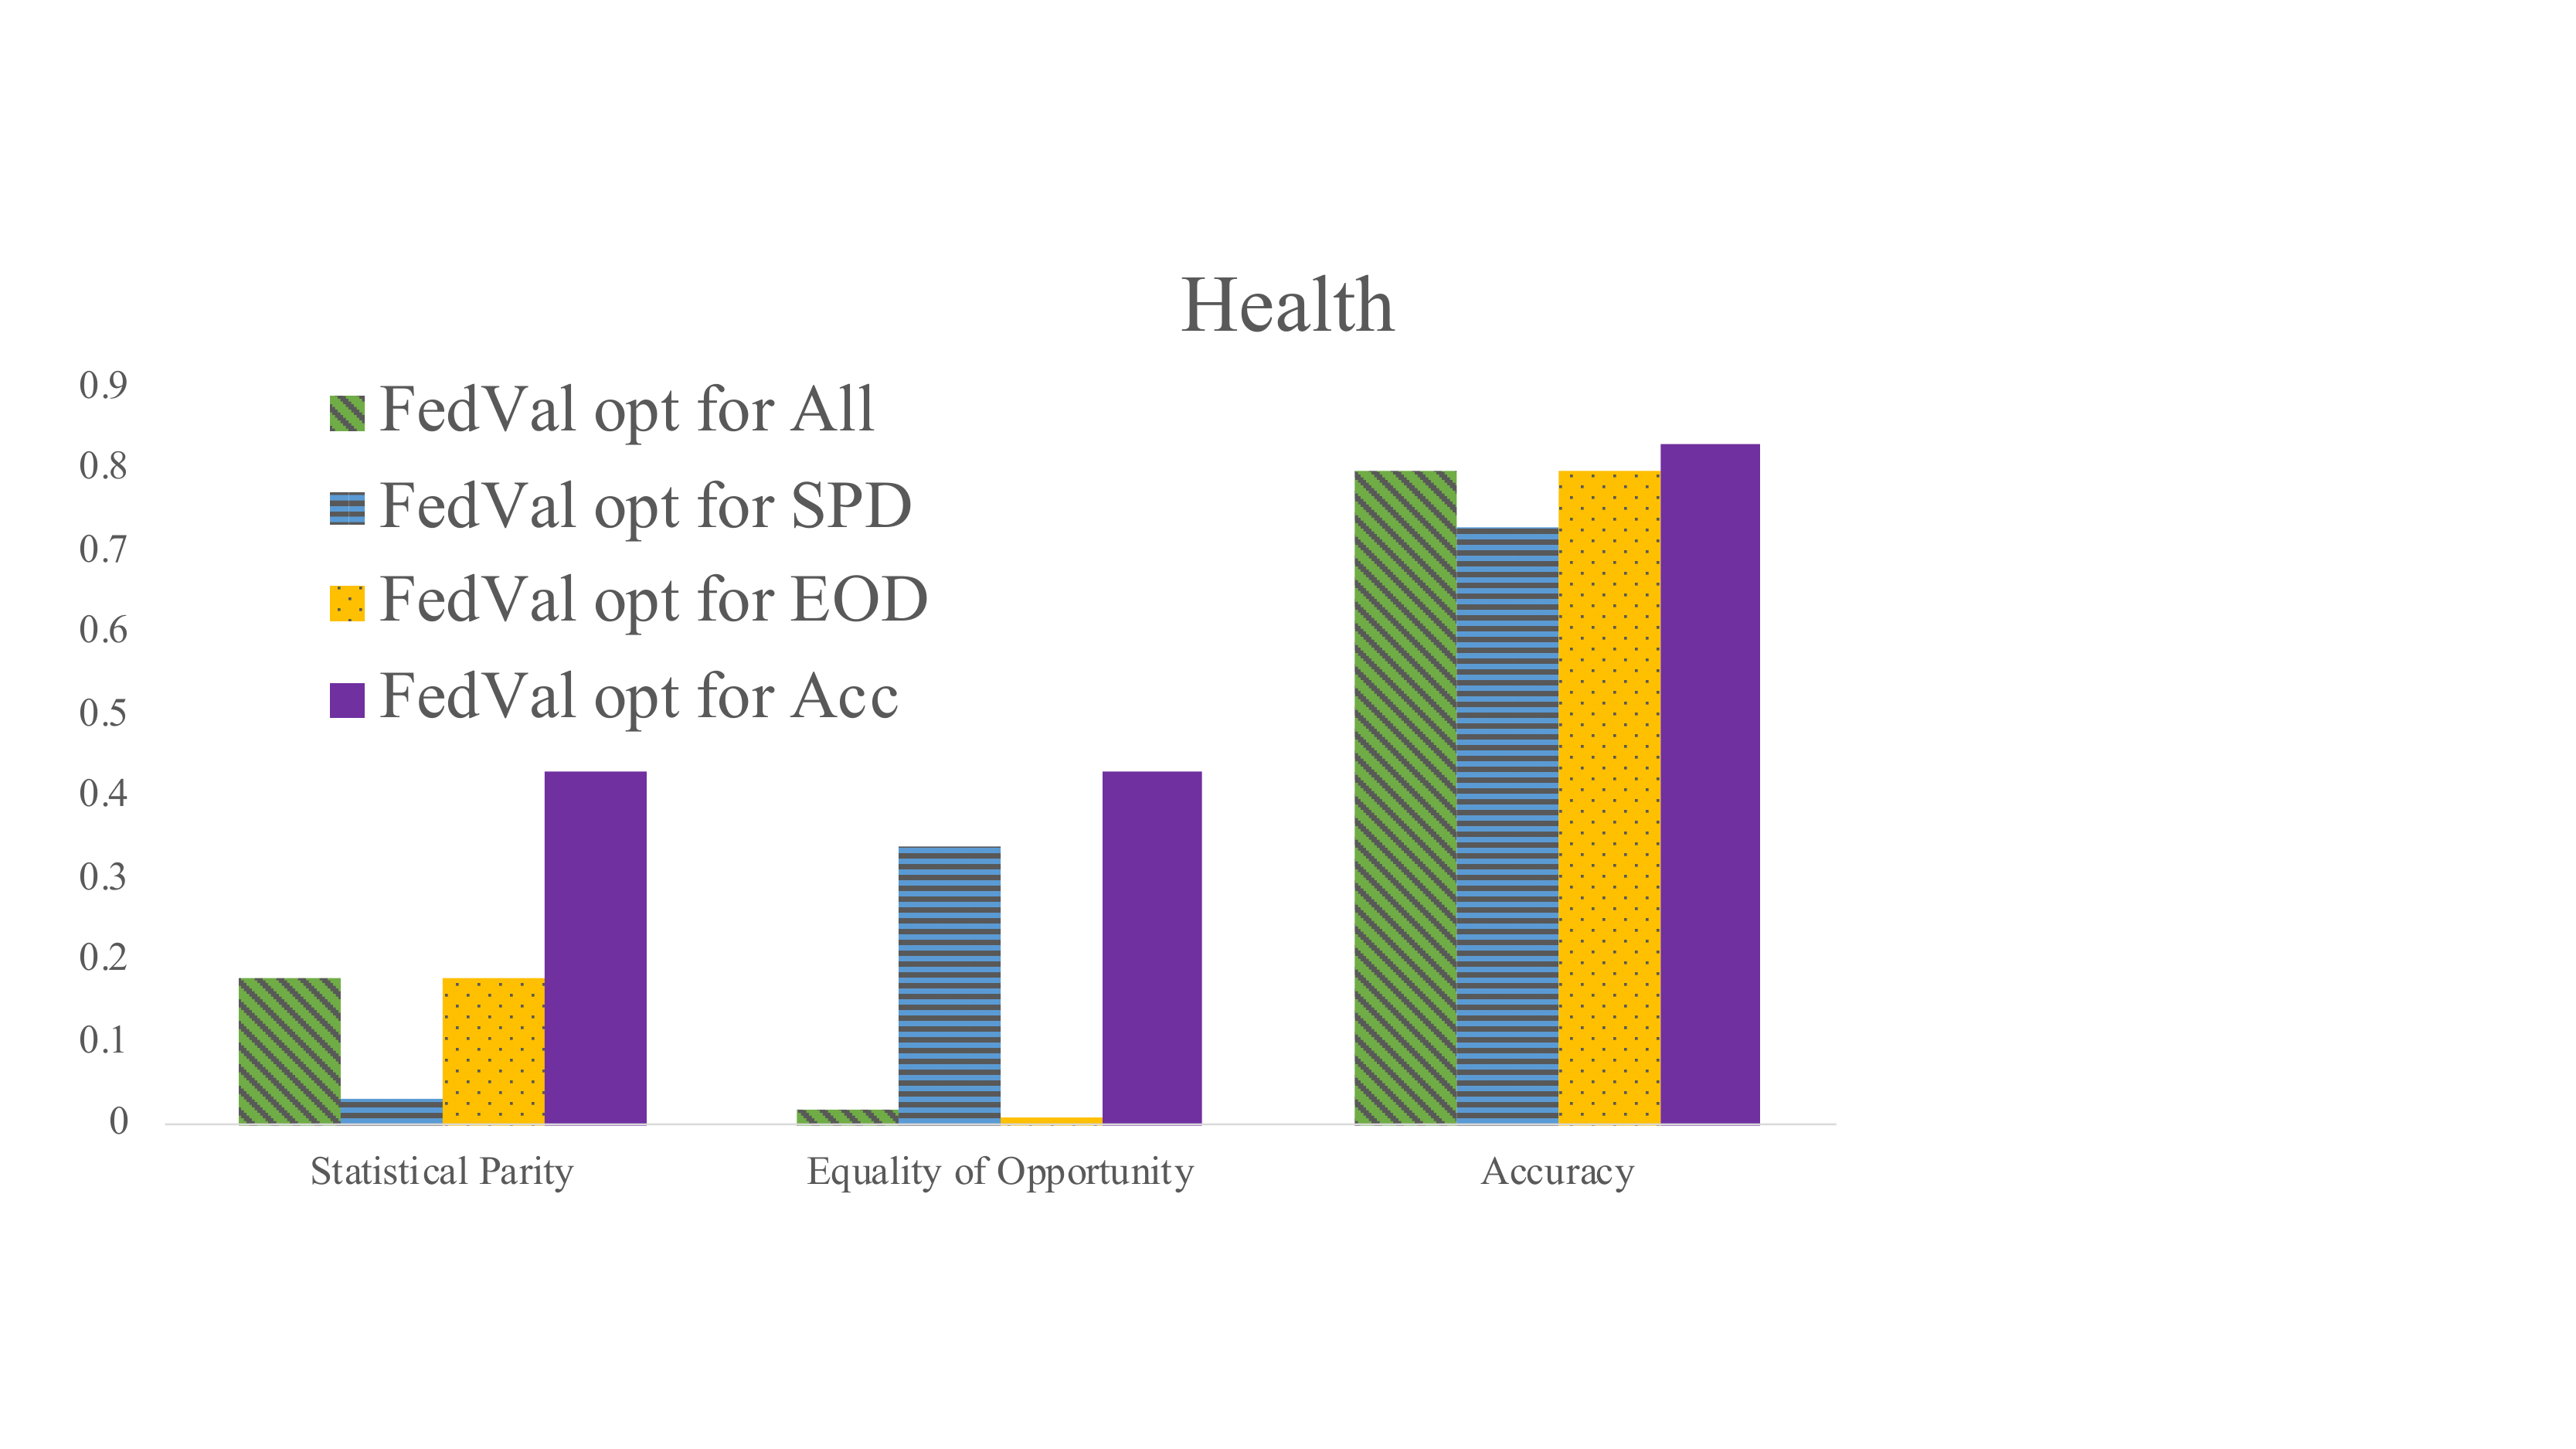}
\caption{FedVal optimized for different objectives in data regime two.}
\label{app-fig5}
\end{figure*}

\begin{figure*}[h]
\includegraphics[width=0.5\textwidth,trim=1cm 3cm 10cm 3cm,clip=true]{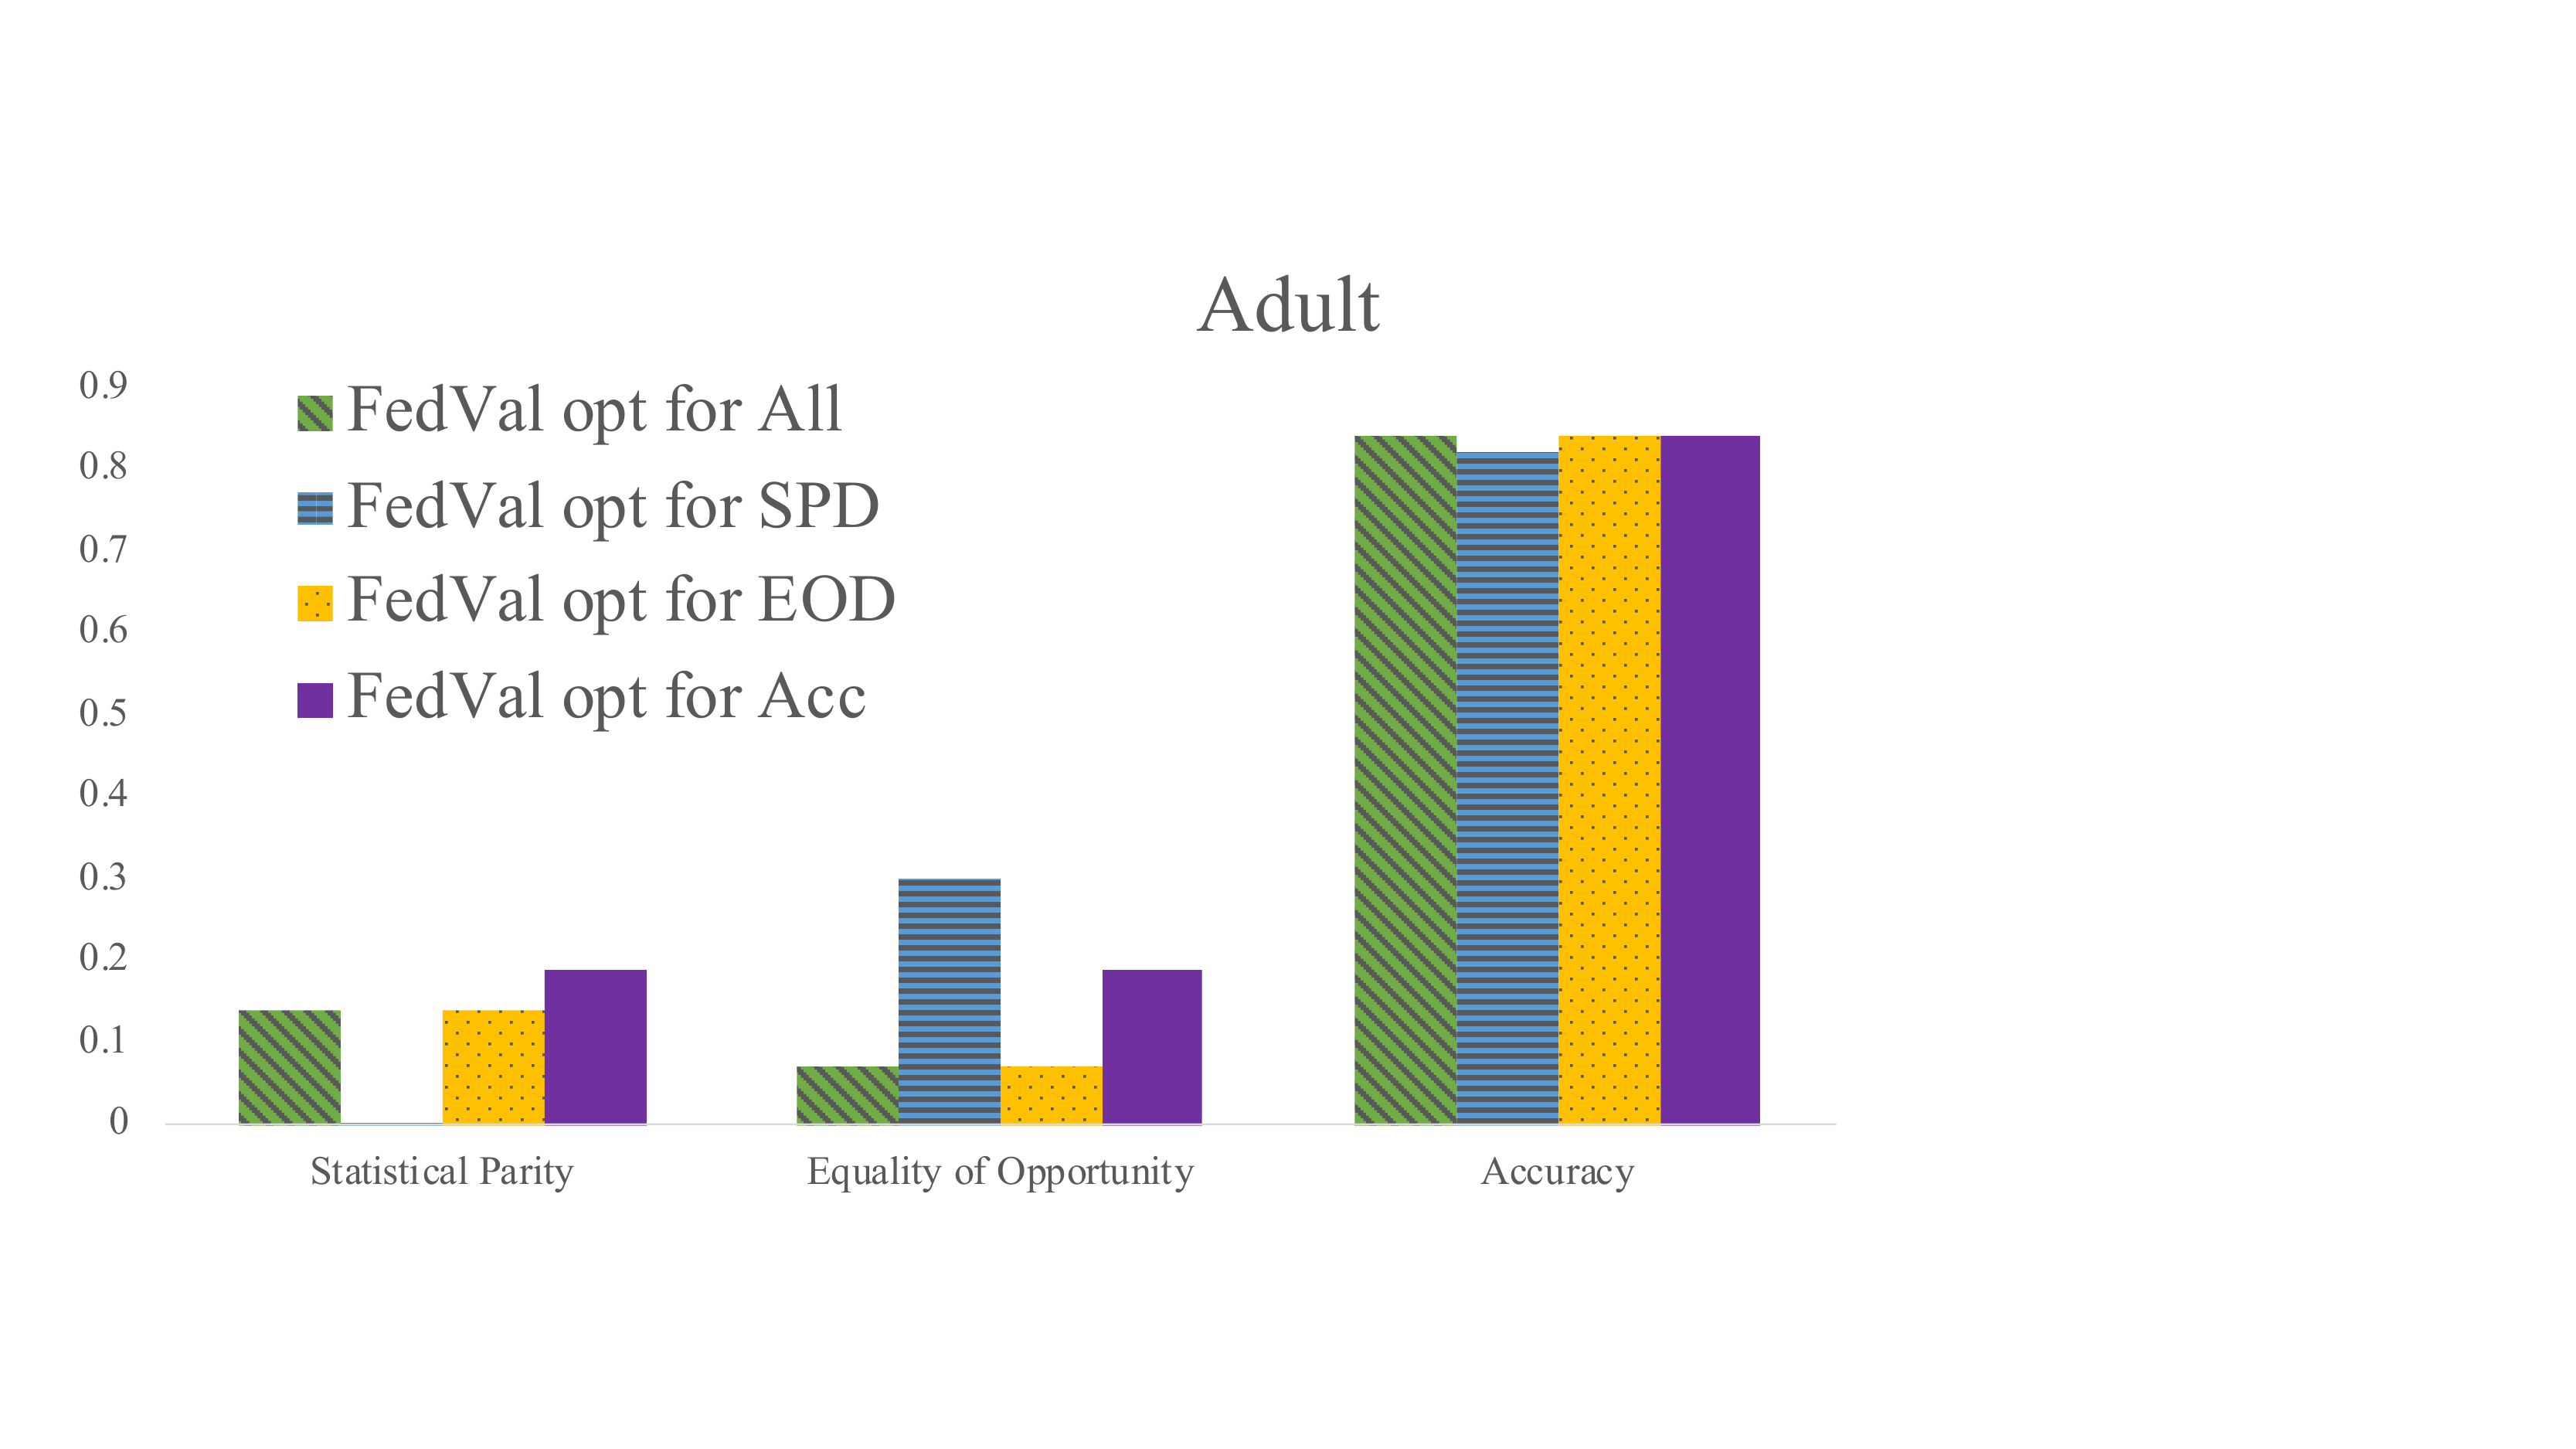}
\includegraphics[width=0.5\textwidth,trim=1cm 3cm 10cm 3cm,clip=true]{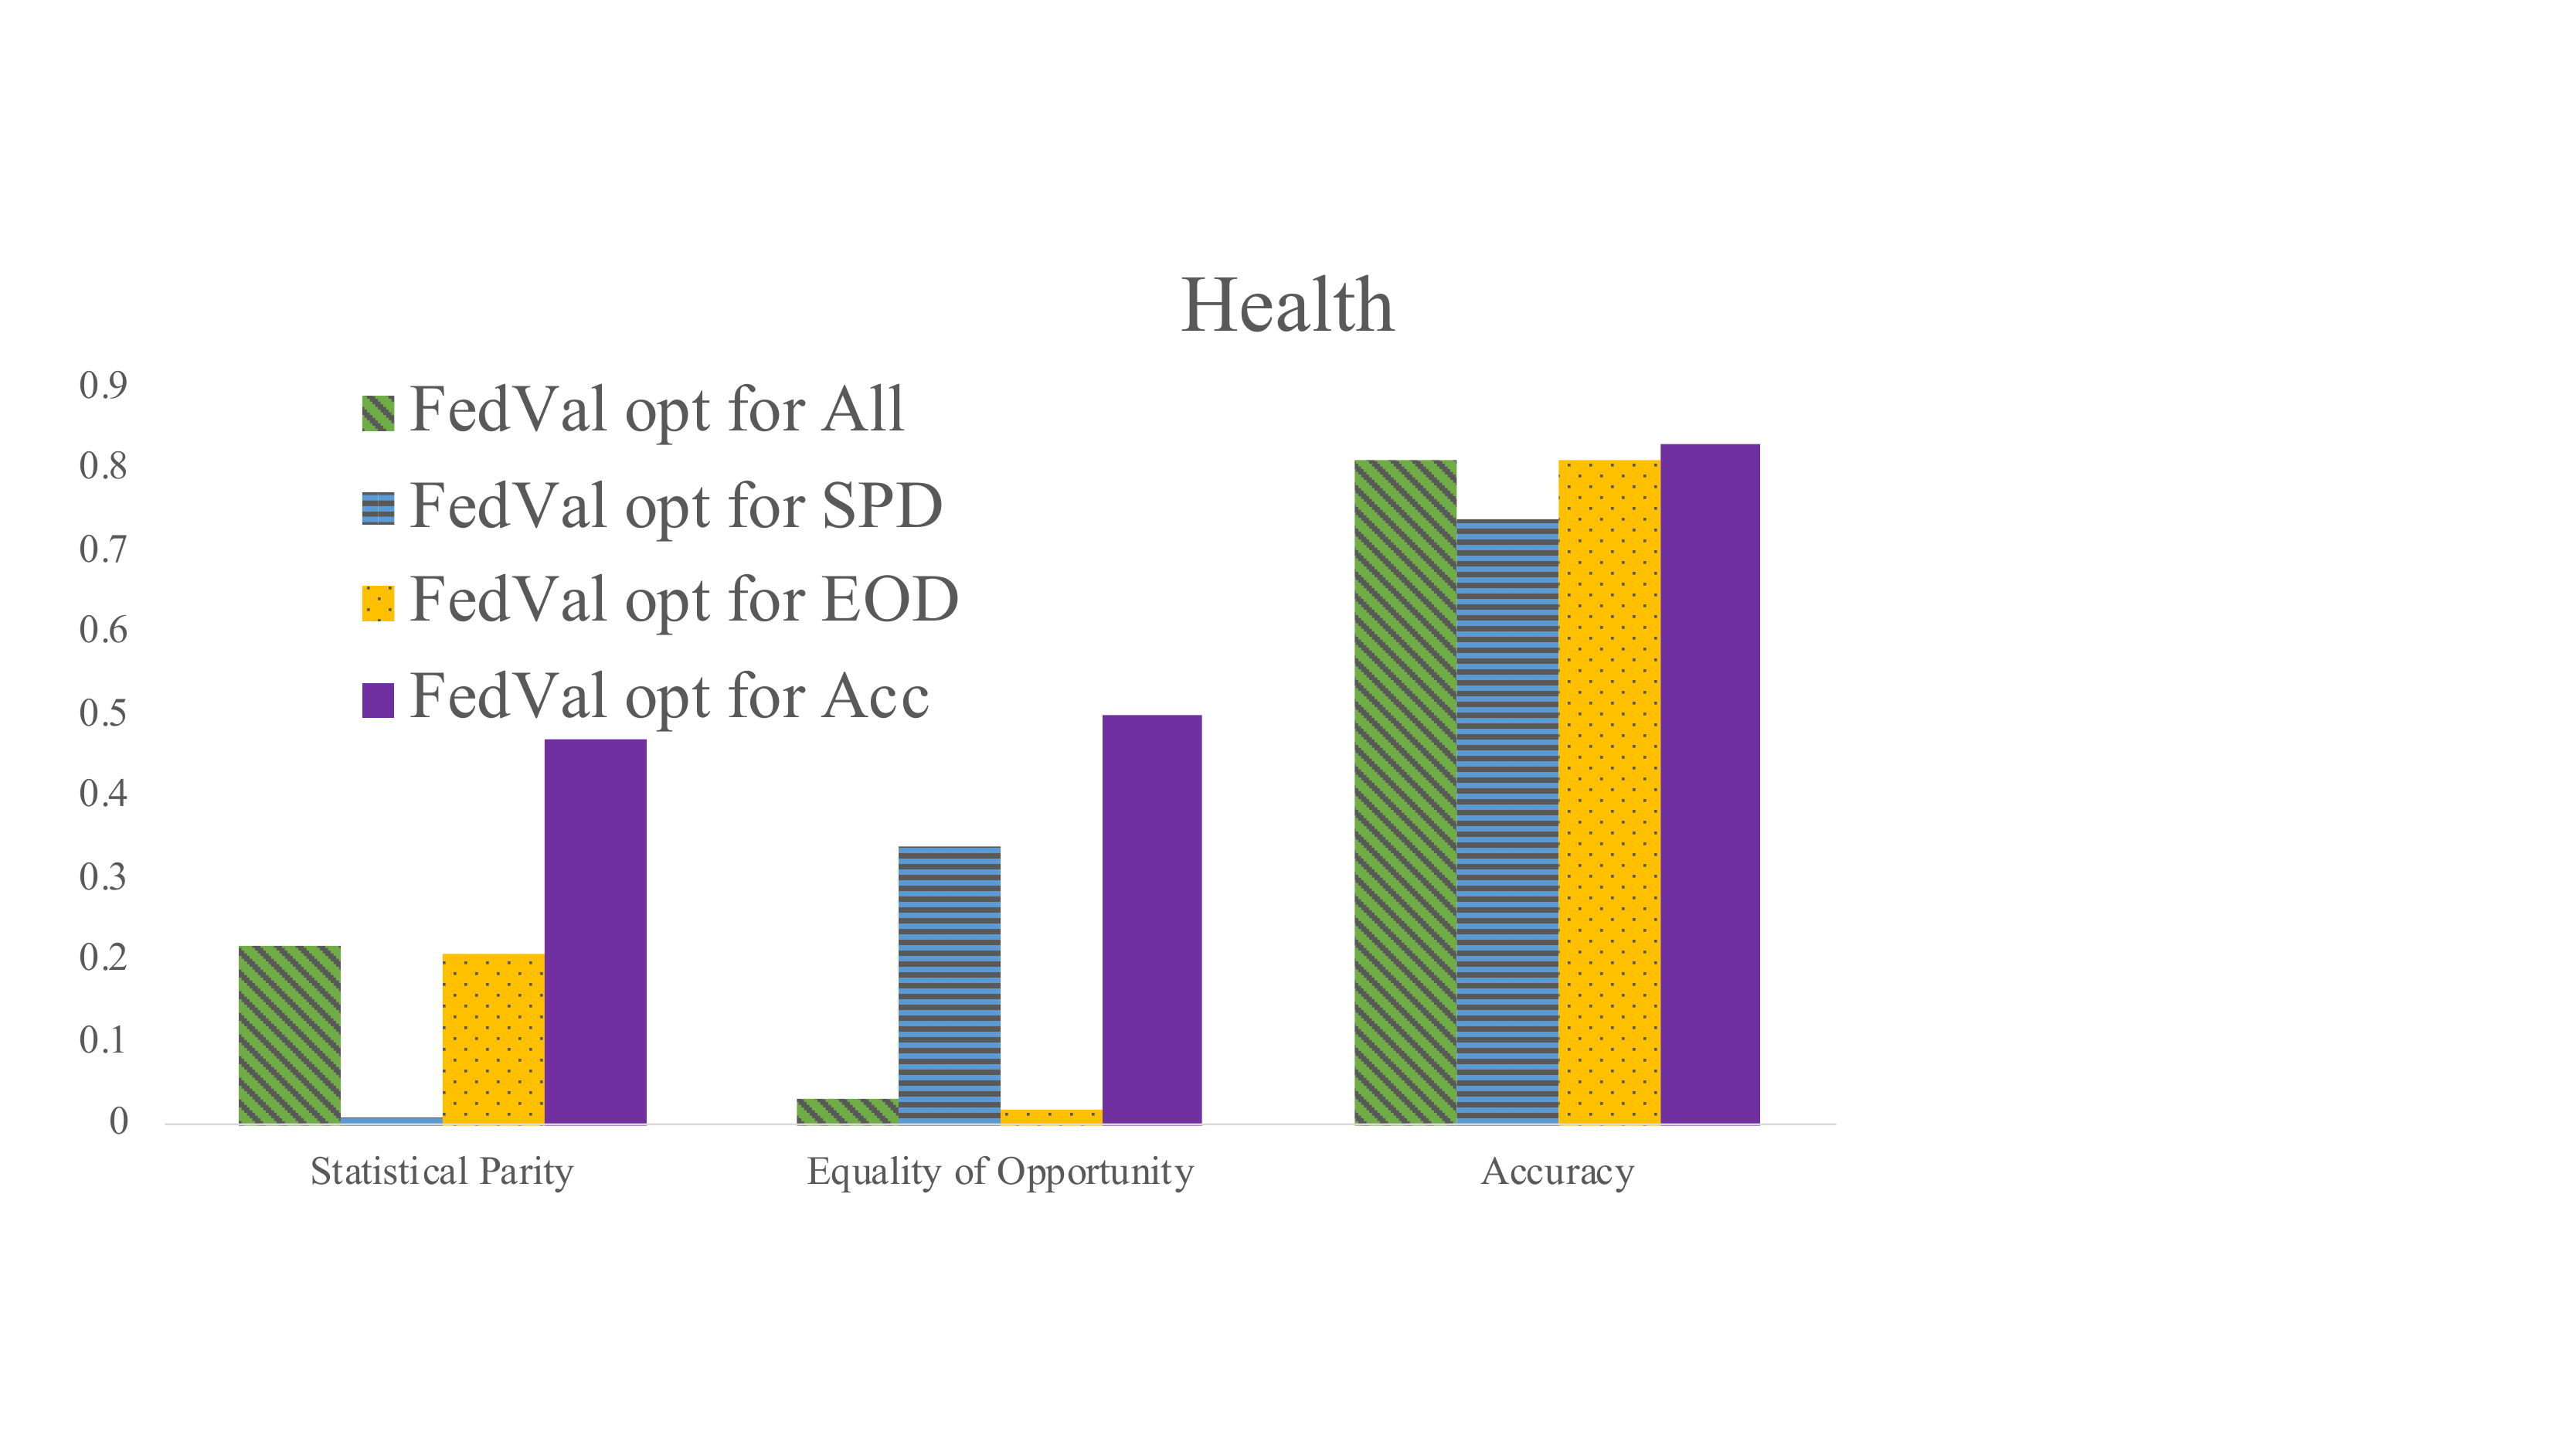}
\caption{FedVal optimized for different objectives in data regime three.}
\label{app-fig6}
\end{figure*}
\clearpage
